# Supplementary material for: Optimal One-pass Nonparametric Estimation Under Memory Constraint
Source: arXiv:2208.08668 source file (2022-08-18)
Supplement: Supplementary file 1 [file supplement.pdf]

# Supplementary Materials to "Optimal One-pass Nonparametric Estimation Under Memory Constraint"

Mingxue Quan Zhenhua Lin

*Organization.* Section S1 provides a proof for Proposition 1, while Sections S2 and S3 respectively contain a proof for Theorems 1 and 2. Technical lemmas are included and proved in Section S4. Section S5 describes the algorithm of the proposed method, while Sections S6 and S7 are devoted to tuning parameter selection and additional simulation studies. Numeric experiments on phase transitions and the smoothness of density function are respectively presented in Sections S8 and S9. Section S10 presents a comparison on computation time. A brief description on Fourier extension is given in Section S11.

*General remarks and additional notation.* For a distribution $F$, we use $\Pr_F$ and $\mathbb{E}_F$ to respectively denote the probability and expectation with respect to the probability measure induced by $F$. For a probability density $f$ on $\mathcal{T}$, $\Pr_f$ and $\mathbb{E}_f$ are understood analogously. In addition, $\mathbb{E}_{\mathcal{T}}$ denotes the expectation with respect to the usual Lebesgue measure on $\mathcal{T}$.

For a random quantity $X_n$, we write $X_n = O_P^{\mathcal{F}}(b_n)$ if

$$\lim_{A\to\infty} \limsup_{n\to\infty} \sup_{F\in\mathcal{F}} \Pr_F(|X_n| \geq Ab_n) = 0.$$

We say the probability of a sequence of events $E_n(A)$ indexed by both $n$ and $A$ converges/decays to zero uniformly over the class $\mathcal{F}$ if

$$\lim_{A\to\infty} \limsup_{n\to\infty} \sup_{F\in\mathcal{F}} \Pr_F\{E_n(A)\} = 0.$$

We may suppress $F$ or $f$ from $\Pr_F$, $\Pr_f$, $\mathbb{E}_F$ and $\mathbb{E}_f$ in the sequel to reduce notational burden unless there is potential confusion.

We write $\phi(t) = (\phi_1(t), \ldots, \phi_q(t))^\top$, $\psi(t) = (\psi_1(t), \ldots, \psi_p(t))^\top$, $\theta = (\theta_1, \ldots, \theta_p)^\top$ and $a = (a_1, \ldots, a_q)^\top$ with $\theta_j = \int_{\mathcal{T}} f(t)\psi_j(t)dt$ for $j = 1, \ldots, p$ and $a_j = \int_{\mathcal{T}} m(t)\phi_j(t)dt$ for $j =$

$1, \dots, q$. Recall that $H_q$ denotes the $q \times q$ matrix formed by the elements $\int_{\mathcal{T}} \phi_j(t)\phi_k(t)f(t)dt$ for $j, k = 1, \dots, q$. The Euclidean norm of a vector is denoted by $\|\cdot\|_2$ and the matrix operator norm with respect to $\|\cdot\|_2$ is denoted by $\|\cdot\|$. We use $I(\cdot)$ to denote the indicator function. By Assumption 3, there exists $\sigma > 0$ such that $\mathbb{E}\varepsilon_i^2 \le \sigma^2$ for all $i = 1, \dots, n$.

Unless otherwise stated, the constants $c, c_1, c_2, \dots$ do not depend on $s$, $t$, $i$, $j$, $k$, $p$, $q$, $n$, $f$, $m$ or $F$; they depend only on the constant $C_*$ in the proofs and other constants in the assumptions of the proposition or theorems. In addition, the value of $c$ is allowed to vary from place to place.

# S1 Proof of Proposition 1

*Proof of Proposition 1.* It is sufficient to prove the proposition for $n \ge 2$. By assumption there exists $C_* > 0$ such that $p^\alpha \log(p+1) \le C_* n$. Let $\hat\theta = (\hat\theta_1, \dots, \hat\theta_p)^\top$ with $\hat\theta_j$ being the $j$th element of the vector $\hat\theta_{1:n}$ defined in Section 2. Let $\check f(t) = (\hat\theta - \theta)^\top \psi(t)$. As in the proof of Lemma 2.3 of Chen and Christensen (2015), by the mean value theorem and the assumption that $\{\psi_j\}_{j=1}^\infty$ is a $(C_\psi, \alpha, \alpha_1)$-basis, we observe

$$\begin{aligned}
|\check f(t) - \check f(t^*)| &= |\{\psi(t) - \psi(t^*)\}^\top (\hat\theta - \theta)| \\
&= |(t - t^*)\nabla\psi(t^{**})^\top (\hat\theta - \theta)| \\
&\le \sqrt{C_\psi} p^{\alpha_1/2} |t - t^*| \cdot \|\hat\theta - \theta\|_2
\end{aligned}$$

for some $t^{**}$ lies between $t$ and $t^*$. Let $\mathscr{B}_n$ be the event that $\|\hat\theta - \theta\|_2 \le A$. We can choose positive constants $\eta_1$ and $\eta_2$ such that, on the event $\mathscr{B}_n$, for any $A \ge 1$,

$$\sqrt{C_\psi} p^{\alpha_1/2} |t - t^*| \|\hat\theta - \theta\|_2 \le A r_n$$

for $r_n = \sqrt{p^\alpha n^{-1} \log(n+1)}$ whenever $|t - t^*| \le \eta_1 n^{-\eta_2}$. This is feasible because of $p \lesssim n^{1/\alpha}$ that is implied by the assumption $p^\alpha \log(p+1) \lesssim n$.

Let $\mathcal{S} \subset \mathcal{T}$ be a smallest subset that covers $\mathcal{T}$ in the sense that to each $t \in \mathcal{T}$, there is $s \in \mathcal{S}$ such that $|s - t| \le \eta_1 n^{-\eta_2}$. Let $s_n(t)$ denote the $s \in \mathcal{S}$ that is closest to $t$. On $\mathscr{B}_n$ we then observe that

$$\sup_{t \in \mathcal{T}} |\check f(t) - \check f(s_n(t))| \le A r_n.$$

Let $\overline{\mathscr{B}}_n$ denote the complement of $\mathscr{B}_n$. By using the simple fact $\Pr(E_1) \le \Pr(E_1 \cap E_2) +$

$\Pr(\overline{E}_2)$ for any events $E_1$ and $E_2$, we deduce that

$$\begin{aligned}
\Pr\big(\|\check{f}\|_\infty \geq 4Ar_n\big) &\leq \Pr\big(\{\|\check{f}\|_\infty \geq 4Ar_n\} \cap \mathscr{B}_n\big) + \Pr(\overline{\mathscr{B}}_n) \\
&\leq \Pr\big(\{\sup_t |\check{f}(t) - \check{f}(s_n(t))| \geq 2Ar_n\} \cap \mathscr{B}_n\big) \\
&\quad + \Pr\big(\{\max_{s\in\mathcal{S}} |\check{f}(s)| \geq 2Ar_n\} \cap \mathscr{B}_n\big) + \Pr(\overline{\mathscr{B}}_n) \\
&= \Pr\big(\{\max_{s\in\mathcal{S}} |\check{f}(s)| \geq 2Ar_n\} \cap \mathscr{B}_n\big) + \Pr(\overline{\mathscr{B}}_n) \\
&\leq \Pr\big(\max_{s\in\mathcal{S}} |\check{f}(s)| \geq 2Ar_n\big) + \Pr(\overline{\mathscr{B}}_n). \qquad \text{(S1)}
\end{aligned}$$

Below we provide bounds for each term in (S1).

Define $\varphi(T_i) = (nn_1^{-1}(\psi_1(T_i) - \theta_1)I(i \geq \tau_1), \ldots, nn_p^{-1}(\psi_p(T_i) - \theta_p)I(i \geq \tau_p))^\top$, where we recall $n_j = n - \tau_j + 1$ for $j = 1, \ldots, p$. By construction, $\hat{\theta} - \theta = n^{-1}\sum_{i=1}^n \varphi(T_i)$. Note that

$$\|\varphi(T_i)\|_2^2 \leq \sum_{j=1}^p 2n^2 n_j^{-2}\{\psi_j^2(T_i) + \theta_j^2\}I(\tau_j \leq i) \leq 2n^2 n_p^{-2}\sum_{j=1}^p \psi_j^2(T_i) + c\|\theta\|_2^2 \leq cp^\alpha, \qquad \text{(S2)}$$

where we use the fact $\|\theta\|_2 \leq c$, $(1 - c_\circ)n \leq n_p \leq n_j \leq n$ and the assumption that $\{\psi_j\}_{j=1}^\infty$ is a $(C_\psi, \alpha)$-basis so that

$$\sup_{s\in\mathcal{T}} \|\psi(s)\|_2^2 \leq C_\psi p^\alpha. \qquad \text{(S3)}$$

Consequently, if we set $Z_i = \psi(s)^\top\varphi(T_i)$ so that $\check{f}(s) = \psi(s)^\top(\hat{\theta} - \theta) = n^{-1}\sum_{i=1}^n Z_i$, then we observe

$$|n^{-1}Z_i| \leq n^{-1}\|\psi(s)\|_2\|\varphi(T_i)\|_2 \leq c_1 p^\alpha/n,$$

where the second inequality is due to (S2) and (S3). In addition,

$$\begin{aligned}
\sum_{i=1}^n \mathbb{E}(n^{-1}Z_i)^2 &= n^{-2}\sum_{i=1}^n \psi(s)^\top\mathbb{E}\{\varphi(T_i)\varphi(T_i)^\top\}\psi(s) \\
&\leq cp^\alpha n^{-2}\sum_{i=1}^n \|\mathbb{E}\{\varphi(T_i)\varphi(T_i)^\top\}\|.
\end{aligned}$$

We claim that $\|\mathbb{E}\{\varphi(T_i)\varphi(T_i)^\top\}\| \leq c$ so that $\sum_{i=1}^n \mathbb{E}(n^{-1}Z_i)^2 \leq c_2 p^\alpha/n$, which follows from

the following derivations: For any $v \in \mathbb{R}^p$ with $v \neq 0$,

$$
\begin{aligned}
|v^\top \mathbb{E}\{\varphi(T_i)\varphi(T_i)^\top\}v| &\le \mathbb{E}|v^\top \varphi(T_i)|^2 \\
&= \sum_{j=1}^{p} I(i \ge \tau_j)\mathbb{E}[v_j n n_j^{-1}\{\psi_j(T_i) - \theta_j\}]^2 \\
&\le c\sum_{j=1}^{p} \mathbb{E}[v_j\{\psi_j(T_i) - \theta_j\}]^2 \\
&\le c\sum_{j=1}^{p} \mathbb{E}_{\mathcal{T}}(v_j\psi_j(T))^2 + c\sum_{j=1}^{p} v_j^2\theta_j^2 \\
&\le c\|v\|_2^2 + c\sum_{j=1}^{p} v_j^2 \\
&\le c\|v\|_2^2, \qquad \text{(S4)}
\end{aligned}
$$

where the second inequality is due to $(1 - c_\circ)n \le n_p \le n_j \le n$, the third is partially based on $\|f\|_\infty \le M$, and the fourth relies on $\|\theta\|_\infty \le \|\theta\|_2 \le c$.

With the observation $\mathbb{E}Z_i = 0$, now we apply Bernstein's inequality to conclude that

$$
\begin{aligned}
\Pr\Big(|\check{f}(s)| \ge \eta r_n\Big) &= \Pr\Big(\Big|\sum_{i=1}^{n} n^{-1}Z_i\Big| \ge \eta r_n\Big) \\
&\le 2\exp\left(-\frac{\eta^2 r_n^2/2}{c_2 p^\alpha/n + c_1\eta p^\alpha r_n/(3n)}\right) \\
&\le c\exp(-c_3\eta\log n) \qquad \text{(S5)}
\end{aligned}
$$

for all $n \ge 1$ and all sufficiently large $\eta > 0$. Noting that the cardinality of $\mathcal{S}$ satisfies $|\mathcal{S}| \le cn^{\eta_2}$, using (S5), we deduce that, for some constant $c_4 > 0$, for all sufficiently large $A$, for all $n \ge 2$,

$$
\begin{aligned}
\Pr\big(\max_{s\in\mathcal{S}} |\check{f}(s)| \ge 2Ar_n\big) &\le |S_n| \max_{s\in\mathcal{S}} \Pr\big(|\check{f}(s)| \ge 2Ar_n\big) \\
&\le cn^{\eta_2}\exp(-2c_3 A\log n) \le cn^{-2c_4 A}. \qquad \text{(S6)}
\end{aligned}
$$

By the assumed condition on $p$, $\sqrt{p^\alpha \log(p+1)}/\sqrt{n} \le 1/c_5$ for a positive constant $c_5$, which implies that $\Pr(\|\hat{\theta} - \theta\|_2 \ge A) \le 2^{-c_5 A/2+1}$ for all sufficiently large $A$ according to Claim 1. This, together with (S1) and (S6), yields $\Pr(\|\check{f}\|_\infty \ge 4Ar_n) \le cn^{-2c_4 A} + c2^{-c_5 A/2}$.

This exponential tail bound in turn implies that, for any $\ell > 0$, $\mathbb{E}\|\check{f}\|_\infty^\ell \le cr_n^\ell$, since $\mathbb{E}\{r_n^{-\ell}\|\check{f}\|_\infty^\ell\} = \int_0^\infty \Pr(r_n^{-1}\|\check{f}\|_\infty \ge A^{1/\ell})dA \le c$. The conclusion of the proposition then follows from $\|\hat{f} - f\|_\infty \le \|\check{f}\|_\infty + \kappa_{\psi,\infty}(p)$.

Now we state and prove the claim referenced in the above to complete the proof of the proposition.

**Claim 1.** *For all sufficiently large $\eta > 0$,*

$$\sup_{n\ge 1}\sup_{f\in\mathcal{D}(\gamma,\chi,M)} \Pr_f\big(\|\hat{\theta}-\theta\|_2 \ge \eta\sqrt{p^\alpha\log(p+1)}/\sqrt{n}\big) \le 2^{-\eta/2+1}.$$

We first recall $\hat{\theta} - \theta = \sum_{i=1}^n n^{-1}\varphi(T_i)$ and $\|n^{-1}\varphi(T_i)\|_2 \le cp^{\alpha/2}/n$ from the above derivations. In addition, $|n^{-2}\mathbb{E}\{\varphi(T_i)^\top\varphi(T_i)\}| \le cp^\alpha/n^2$ and $\|n^{-2}\mathbb{E}\{\varphi(T_i)\varphi(T_i)^\top\}\| \le cn^{-2}$ based on (S4). According to Corollary 3.1 of Minsker (2017) or Lemma D.4 of Ding and Zhou (2020), we then have

$$\begin{aligned}\Pr_f(\|\hat{\theta}-\theta\|_2 \ge s) &= \Pr_f\left(\left\|\sum_{i=1}^n n^{-1}\varphi(T_i)\right\|_2 \ge s\right)\\ &\le (p+1)\exp\left(\frac{-s^2/2}{cp^\alpha/n + cp^{\alpha/2}s/(3n)}\right).\end{aligned}$$

Taking $s = \eta\sqrt{p^\alpha\log(p+1)}/\sqrt{n}$ in the above, we conclude that

$$\Pr_f\big(\|\hat{\theta}-\theta\|_2 \ge \eta\sqrt{p^\alpha\log(p+1)}/\sqrt{n}\big) \le (p+1)^{-\eta/2+1} \le 2^{-\eta/2+1}$$

for all $\eta \ge \eta_0$ for a sufficiently large positive constant $\eta_0$ that is independent of $n$, $p$ and $f$, since $\log(p+1) \lesssim n$ is assumed. Since all the constants do not depend on $f$ and $n$, this proves the claim. □

## S2 Proof of Theorem 1

*Proof of Theorem 1.* By the assumed conditions on $p$, $q$ and $\rho$, there is a constant $C_*$ such that $p^\alpha \le C_*(n/\log n)^{1/2}$, $q^\alpha \le C_*(n/\log n)^{\xi/(2+\xi)}$, $q^\alpha \le C_*(n/\log n)^{1/2}$, $\kappa_{\psi,\infty}(p) \le C_*$, $\kappa_{\phi,\infty}(q) \le C_*$ and $\rho \le C_*\sqrt{(\log n)/(q^{2\zeta}n)}$. Note that the bounds on $q^\alpha$ and $\rho$ imply $\rho \lesssim q^{-\alpha-\zeta}$. In addition, $\alpha > 0$ and the condition $p^\alpha \le C_*(n/\log n)^{1/2}$ imply $r_n \ll 1$.

We start with defining $\acute{a} = (H_q + \rho W)^{-1}(N_q^{-1}G_q)$ and recalling that $\hat{a} = (\hat{H}_q +$

$\rho W)^{-1}(N_q^{-1}G_q)$. Let $\acute{m}(t) = \acute{a}^\top\phi(t)$ and $\check{m}(t) = (\acute{a}-a)^\top\phi(t)$. By the mean value theorem and the assumption that $\{\phi_j\}_{j=1}^\infty$ is a $(C_\phi, \alpha, \alpha_1)$-basis,

$$
\begin{aligned}
|\check{m}(t) - \check{m}(t^*)| &= |\{\phi(t) - \phi(t^*)\}^\top(\acute{a} - a)| \\
&= |(t - t^*)\nabla\phi(t^{**})^\top(\acute{a} - a)| \\
&\le \sqrt{C_\phi}q^{\alpha_1/2}|t - t^*|\|\acute{a} - a\|_2,
\end{aligned}
$$

where $t^{**}$ lies between $t$ and $t^*$. Let $\mathscr{B}_n$ be an event on which $\sqrt{C_\phi}\|\acute{a} - a\|_2 \le A$ for any fixed $A > 0$. There exist constants $\eta_1$ and $\eta_2$ such that on $\mathscr{B}_n$, for all $A \ge 1$,

$$
\sqrt{C_\phi}q^{\alpha_1/2}|t - t^*|\|\acute{a} - a\|_2 \le A\sqrt{\frac{q^\alpha \log n}{n}} := AR_n,
$$

whenever $|t - t^*| \le \eta_1 n^{-\eta_2}$; this is feasible due to $q^\alpha \le C_*(n/\log n)^{1/2}$.

Let $\mathcal{S}$ be a smallest subset of $\mathcal{T}$ satisfying that, for each $t \in \mathcal{T}$, there exists an $s \in \mathcal{S}$ such that $|s - t| \le \eta_1 n^{-\eta_2}$. If $s_n(t)$ denotes the $s \in \mathcal{S}$ that is closest to $t$, then on the event $\mathscr{B}_n$, we have

$$
\sup_{t\in\mathcal{T}} |\check{m}(t) - \check{m}(s_n(t))| \le AR_n. \tag{S7}
$$

Let $\overline{\mathscr{B}}_n$ denote the complement of $\mathscr{B}_n$. Define $\tilde{R}_n = R_n + (1 + \|\Pi_q^\phi\|_\infty)\kappa_{\phi,\infty}(q)$. According to the simple fact $\Pr(E_1) \le \Pr(E_1 \cap E_2) + \Pr(\overline{E}_2)$ for any two events $E_1$ and $E_2$, we deduce

$$
\begin{aligned}
\Pr(\|\check{m}\|_\infty \ge 8A\tilde{R}_n) &\le \Pr(\{\|\check{m}\|_\infty \ge 8A\tilde{R}_n\} \cap \mathscr{B}_n) + \Pr(\overline{\mathscr{B}}_n) \\
&\le \Pr(\{\sup_{t\in\mathcal{T}} |\check{m}(t) - \check{m}(s_n(t))| \ge 4A\tilde{R}_n\} \cap \mathscr{B}_n) \\
&\quad + \Pr(\{\max_{s\in\mathcal{S}} |\check{m}(s)| \ge 4A\tilde{R}_n\} \cap \mathscr{B}_n) + \Pr(\overline{\mathscr{B}}_n) \\
&= \Pr(\{\max_{s\in\mathcal{S}} |\check{m}(s)| \ge 4A\tilde{R}_n\} \cap \mathscr{B}_n) + \Pr(\overline{\mathscr{B}}_n) \\
&\le \Pr(\{\max_{s\in\mathcal{S}} |\check{m}(s)| \ge 4A\tilde{R}_n\}) \qquad \text{(S8)} \\
&\quad + \Pr(\overline{\mathscr{B}}_n), \qquad \text{(S9)}
\end{aligned}
$$

where the equality is due to (S7).

We first study the probability (S8). Let $\Psi_i(v) = n(n_1^{-1}v_1 I(i \ge \tau_1), \ldots, n_q^{-1}v_q I(i \ge \tau_q))^\top$

for a vector $v \in \mathbb{R}^q$. Note that $n^{-1}\sum_{i=1}^n \Psi_i(v) = v$ if $v$ is not dependent on $i$. Define

$$\begin{aligned}
\varphi(T_i) &= \Psi_i(\phi(T_i)) \\
\varphi_1(T_i) &= \varphi(T_i)(\phi(T_i)^\top a) - \Psi_i(H_q a) \\
\varphi_2(T_i) &= \varphi(T_i)(m(T_i) - \phi(T_i)^\top a) - \Psi_i(\mathbb{E}\{\phi(T)(m(T) - \phi(T)^\top a)\}) \\
\varphi_3(T_i) &= \varepsilon_i \varphi(T_i).
\end{aligned}$$

Note that $\varphi_1, \varphi_2, \varphi_3$ are all centered. Define $Z_i^{(k)} = \phi(s)^\top (H_q + \rho W)^{-1} \varphi_k(T_i)$ for $k = 1, 2, 3$. Then

$$\begin{aligned}
\check{m}(s) =& n^{-1}\sum_{i=1}^n Z_i^{(1)} + n^{-1}\sum_{i=1}^n Z_i^{(2)} + n^{-1}\sum_{i=1}^n Z_i^{(3)} \\
& - \phi(s)^\top (H_q + \rho W)^{-1}(\rho W a) \\
& + \phi(s)^\top (H_q + \rho W)^{-1}\mathbb{E}\{\phi(T)(m(T) - \phi(T)^\top a)\}.
\end{aligned} \tag{S10}$$

Noting that the condition $\rho \lesssim \sqrt{(\log n)/(q^{2\zeta} n)}$ implies $\rho q^{\alpha/2+\zeta} \lesssim R_n$, we deduce that, for all sufficiently large $A$,

$$\begin{aligned}
\sup_{s\in\mathcal{T}} |\phi(s)^\top (H_q + \rho W)^{-1}(\rho W a)| &\leq \rho \sup_{s\in\mathcal{T}} \|\phi(s)\|_2 \|(H_q + \rho W)^{-1}\| \|W\| \|a\|_2 \\
&\leq c\rho q^{\alpha/2+\zeta} \leq A R_n,
\end{aligned} \tag{S11}$$

where the last inequality is based on Lemma 1, Assumption 5 and the assumption that $\{\phi_j\}_{j=1}^\infty$ is a $(C_\phi, \alpha, \alpha_1)$-basis so that

$$\sup_{s\in\mathcal{T}} \|\phi(s)\|_2^2 \leq C_\phi q^\alpha. \tag{S12}$$

In addition, we observe

$$\begin{aligned}
&\sup_{s\in\mathcal{T}} |\phi(s)^\top (H_q + \rho W)^{-1}\mathbb{E}\{\phi(T)(m(T) - \phi(T)^\top a)\}| \\
&\leq \sup_{s\in\mathcal{T}} |\phi(s)^\top \{(H_q + \rho W)^{-1} - H_q^{-1}\}\mathbb{E}\{\phi(T)(m(T) - \phi(T)^\top a)\}| + \|\Pi_q^\phi (m - \phi^\top a)\|_\infty \\
&\leq \sup_{s\in\mathcal{T}} \|\phi(s)\|_2 \|(H_q + \rho W)^{-1} - H_q^{-1}\| \|\mathbb{E}\{\phi(T)(m(T) - \phi(T)^\top a)\}\|_2 + \|\Pi_q^\phi\|_\infty \|m - \phi^\top a\|_\infty \\
&\leq c q^{\alpha/2}\rho q^\zeta \{\mathbb{E}\|\phi(T)(m(T) - \phi(T)^\top a)\|_2^2\}^{1/2} + \|\Pi_q^\phi\|_\infty \kappa_{\phi,\infty}(q) \\
&\leq c q^{\alpha/2}\rho q^\zeta \{\|m - \phi^\top a\|_\infty^2 \mathbb{E}\|\phi(T)\|_2^2\}^{1/2} + \|\Pi_q^\phi\|_\infty \kappa_{\phi,\infty}(q)
\end{aligned}$$

$$
\begin{aligned}
&\le cq^{\alpha+\zeta}\rho\kappa_{\phi,\infty}(q) + \|\Pi_q^{\phi}\|_\infty \kappa_{\phi,\infty}(q) \\
&\le c(1 + \|\Pi_q^{\phi}\|_\infty)\kappa_{\phi,\infty}(q), \qquad \text{(S13)}
\end{aligned}
$$

where $\|(H_q + \rho W)^{-1} - H_q^{-1}\| \le c\rho q^{\zeta}$ is used in deriving the third inequality, the fifth inequality is due to $\mathbb{E}\|\phi(T)\|_2^2 \le \sup_{s\in\mathcal{T}} \|\phi(s)\|_2^2 \le cq^{\alpha}$ according to (S12), and the last one is based on the bound $\rho \lesssim q^{-\alpha-\zeta}$. The bound $\|(H_q + \rho W)^{-1} - H_q^{-1}\| \le c\rho q^{\zeta}$ is based on the observation that $\|(H_q+\rho W)^{-1} - H_q^{-1}\| \le \|(H_q+\rho W)^{-1}\| + \|H_q^{-1}\| \le c$ according to Lemma 1 for all $q$ and that $\|(H_q + \rho W)^{-1} - H_q^{-1}\| = \|\{I_q - H_q^{-1}(\rho W)\}^{-1} H_q^{-1}(\rho W)H_q^{-1}\| \le c\rho q^{\zeta}$ for all sufficiently large $q$ so that $\|H_q^{-1}(\rho W)\| \le 1/2$ due to $\rho q^{\zeta} \lesssim \sqrt{(\log n)/n} \ll 1$, where $I_q$ denotes the $q \times q$ identity matrix.

Given the bounds (S10), (S11) and (S13), we further deduce that, for all sufficiently large $A$,

$$
\begin{aligned}
\Pr(\{\max_{s\in\mathcal{S}} |\check{m}(s)| \ge 4A\tilde{R}_n\}) &\le \Pr(\{\max_{s\in\mathcal{S}} |n^{-1}\sum_{i=1}^n Z_i^{(1)}| \ge AR_n\}) && \text{(S14)} \\
&\quad + \Pr(\{\max_{s\in\mathcal{S}} |n^{-1}\sum_{i=1}^n Z_i^{(2)}| \ge AR_n\}) && \text{(S15)} \\
&\quad + \Pr(\{\max_{s\in\mathcal{S}} |n^{-1}\sum_{i=1}^n Z_i^{(3)}| \ge AR_n\}). && \text{(S16)}
\end{aligned}
$$

Together with Claims 2–4, the above result implies that the probability (S8) decays to zero uniformly over the class $\mathcal{F}$.

Now we consider the probability $\Pr(\overline{\mathscr{B}}_n) = \Pr(\sqrt{C_\phi}\|\acute{a} - a\|_2 \ge A)$ in (S9). Noting that the assumed condition on the rate of $q$ implies $q^{\alpha} \le cn$, using Lemmas 1 and 3, we deduce that

$$
\begin{aligned}
\sup_{F\in\mathcal{F}} \mathbb{E}_F(\|\acute{a} - a\|_2) &\le \sup_{F\in\mathcal{F}} \mathbb{E}_F\|\acute{a}\|_2 + cM \\
&= \sup_{F\in\mathcal{F}} \mathbb{E}_F\|(H_q + \rho W)^{-1}(N_q^{-1}G_q)\|_2 + cM \\
&\le c\sup_{F\in\mathcal{F}} \mathbb{E}_F\|N_q^{-1}G_q\|_2 + cM \\
&\le c(1 + q^{\alpha}/n) \\
&\le c.
\end{aligned}
$$

Consequently, Markov's inequality implies that, when $A$ is sufficiently large, $\Pr(\overline{\mathscr{B}}_n)$ decays to zero uniformly over the class $\mathcal{F}$. In summary, $\Pr(\|\check{m}\|_\infty \geq 8A\tilde{R}_n)$ decays to zero uniformly over the class $\mathcal{F}$, or equivalently,

$$\lim_{A\to\infty} \limsup_{n\to\infty} \sup_{F\in\mathcal{F}} \Pr_F(\|\acute{m} - \phi^\top a\|_\infty \geq A\tilde{R}_n) = 0. \tag{S17}$$

Given (S17) and Claim 7, the theorem follows from $\|\hat{m}-m\|_\infty \leq \|\hat{m}-\acute{m}\|_\infty + \|\acute{m}-\phi^\top a\|_\infty + \|\phi^\top a - m\|_\infty$ and $\|\phi^\top a - m\|_\infty \leq \kappa_{\phi,\infty}(q)$, where we note that $\|\hat{m} - \acute{m}\|_\infty = 0$ when $f$ is known.

Below we state and prove the claims referenced in the above to complete the proof of the theorem.

**Claim 2.** *The probability* (S14) *decays to zero uniformly over the class* $\mathcal{F}$*.*

We first observe

$$\begin{aligned}
\Big|\frac{1}{n}Z_i^{(1)}\Big| &= \frac{1}{n}|\phi(s)^\top (H_q + \rho W)^{-1}\varphi_1(T_i)| \\
&= \frac{1}{n}|\phi(s)^\top (H_q + \rho W)^{-1}\{(\phi(T_i)^\top a)\varphi(T_i) - \Psi_i(H_q a)\}| \\
&\leq \frac{cq^{\alpha/2}}{n}\|(\phi(T_i)^\top a)\varphi(T_i) - \Psi_i(H_q a)\|_2 \\
&\leq \frac{cq^{\alpha/2}}{n}\{\|\phi^\top a\|_\infty \|\varphi(T_i)\|_2 + \|\Psi_i(H_q a)\|_2\} \\
&\leq c_1 q^\alpha / n,
\end{aligned}$$

where the first inequality is due to (S12) and Lemma 1, and the last inequality is based on Claim 5 and $\|\phi^\top a\|_\infty = \|m\|_\infty + \|m - \phi^\top a\|_\infty \leq c$.

In addition, we find that

$$\begin{aligned}
\sum_{i=1}^n \mathbb{E}\Big\{\frac{1}{n}Z_i^{(1)}\Big\}^2 &= \frac{1}{n^2}\sum_{i=1}^n \phi(s)^\top (H_q + \rho W)^{-1} B_i (H_q + \rho W)^{-1}\phi(s) \\
&\leq \frac{c}{n^2}\sum_{i=1}^n \|B_i\| \|\phi(s)\|_2^2 \\
&\leq \frac{c}{n^2}\sum_{i=1}^n q^\alpha
\end{aligned}$$

$$= \frac{c_2 q^\alpha}{n},$$

where $B_i = \mathbb{E}\big\{[\varphi(T_i)\phi(T_i)^\top a - \Psi_i(H_q a)][\varphi(T_i)\phi(T_i)^\top a - \Psi_i(H_q a)]^\top\big\}$ and we use the fact that $B_1, \ldots, B_n$ have a uniformly bounded operator norm according to Claim 6. Bernstein's inequality then asserts that

$$\Pr\bigg(\max_{s\in\mathcal{S}}\Big|\sum_{i=1}^n \frac{1}{n} Z_i^{(1)}\Big| \geq AR_n\bigg) \leq |\mathcal{S}| \max_{s\in\mathcal{S}} \exp\left(-\frac{A^2 R_n^2/2}{c_2 q^\alpha/n + c_1 q^\alpha AR_n/(3n)}\right)$$
$$\leq cn^{\eta_2} \exp\left(-\frac{A^2 \log n}{2c_2 + (2c_1/3)AR_n}\right).$$

The assumed condition on the rate of $q$ implies $R_n \leq c$, and consequently the above inequality implies that $\Pr(\max_{s\in\mathcal{S}} |\frac{1}{n}\sum_{i=1}^n Z_i^{(1)}| \geq AR_n)$ decays to zero uniformly over the class $\mathcal{F}$.

**Claim 3.** *The probability (S15) decays to zero uniformly over the class $\mathcal{F}$.*

Let $g(t) = \phi(t)\{m(t) - \phi(t)^\top a\}$. We start with the observation

$$\begin{aligned}
\big|\frac{1}{n} Z_i^{(2)}\big| &= \frac{1}{n}|\phi(s)^\top (H_q + \rho W)^{-1}\varphi_2(T_i)| \\
&\leq \frac{1}{n}|\phi(s)^\top (H_q + \rho W)^{-1}\varphi(T_i)| \cdot |m(T_i) - \phi^\top(T_i)a| \\
&\quad + \frac{c}{n}\|\phi(s)\|_2 \|(H_q + \rho W)^{-1}\| \|\mathbb{E}g(T)\|_2 \\
&\leq \frac{\kappa_{\phi,\infty}(q)}{n}\|\phi(s)\|_2\|(H_q + \rho W)^{-1}\|\{\|\varphi(T_i)\|_2 + (\mathbb{E}\|\phi(T)\|_2^2)^{1/2}\} \\
&\leq c_3 q^\alpha/n,
\end{aligned}$$

where the last inequality is due to Lemma 1, $\kappa_{\phi,\infty}(q) \leq c$, the inequality (S12), and Claim 5. In addition, we find that

$$\begin{aligned}
\sum_{i=1}^n \mathbb{E}\big\{\frac{1}{n} Z_i^{(2)}\big\}^2 &\leq \frac{1}{n^2}\sum_{i=1}^n \|m - \phi^\top a\|_\infty^2 \phi(s)^\top (H_q + \rho W)^{-1}\mathbb{E}\{\varphi(T_i)\varphi(T_i)^\top\}(H_q + \rho W)^{-1}\phi(s) \\
&\quad - \frac{1}{n^2}\sum_{i=1}^n \phi(s)^\top (H_q + \rho W)^{-1}\{\Psi_i(\mathbb{E}g(T))\Psi_i(\mathbb{E}g(T))^\top\}(H_q + \rho W)^{-1}\phi(s) \\
&\leq \frac{c\kappa_{\phi,\infty}^2(q)}{n^2}\sum_{i=1}^n \|\phi(s)\|_2^2 \|\mathbb{E}\{\varphi(T_i)\varphi(T_i)^\top\}\|
\end{aligned}$$

$$\leq c_4 q^\alpha / n,$$

where the second inequality is based on Lemma 1, and the last one is due to (S12), Claim 6 and the assumption $\kappa_{\phi,\infty}(q) \leq c$. Note that $\mathbb{E}Z_i^{(2)} = 0$. Now Bernstein's inequality asserts that

$$\begin{aligned}
\Pr\left(\max_{s\in\mathcal{S}}\left|\sum_{i=1}^n \frac{1}{n} Z_i^{(2)}\right| \geq AR_n\right) &\leq |\mathcal{S}| \max_{s\in\mathcal{S}} \exp\left(-\frac{A^2R_n^2/2}{c_4q^\alpha/n + c_3 q^\alpha AR_n/3n}\right) \\
&\leq cn^{\eta_2} \exp\left(-\frac{A^2\log n}{2c_4 + (2c_3/3)AR_n}\right).
\end{aligned}$$

The assumed condition on the rate of $q$ implies $R_n \leq c$, and consequently the above inequality implies that $\Pr(\max_{s\in\mathcal{S}}|\frac{1}{n}\sum_{i=1}^n Z_i^{(2)}| \geq AR_n)$ decays to zero uniformly over the class $\mathcal{F}$.

**Claim 4.** *The probability* (S16) *decays to zero uniformly over the class* $\mathcal{F}$.

To establish the claim, with an increasing sequence $L_n$ diverging to $\infty$, we define

$$\varepsilon_{1,i,n} = \varepsilon_i I(|\varepsilon_i| \leq L_n) - \mathbb{E}[\varepsilon_i I(|\varepsilon_i| \leq L_n)],$$

and

$$\varepsilon_{2,i,n} = \varepsilon_i - \varepsilon_{1,i,n}.$$

With $Z_{1,i}^{(3)} = \phi(s)^\top (H_q + \rho W)^{-1}\varphi(T_i)\varepsilon_{1,i,n}$ and $Z_{2,i}^{(3)} = \phi(s)^\top (H_q + \rho W)^{-1}\varphi(T_i)\varepsilon_{2,i,n}$, we have the decomposition $Z_i^{(3)} = Z_{1,i}^{(3)} + Z_{2,i}^{(3)}$, and see that the probability (S16) is bounded by $\Pr(\max_{s\in\mathcal{S}}|\sum_{i=1}^n \frac{1}{n}Z_{1,i}^{(3)}| \geq AR_n/2) + \Pr(\max_{s\in\mathcal{S}}|\sum_{i=1}^n \frac{1}{n}Z_{2,i}^{(3)}| \geq AR_n/2)$.

For $\Pr(\max_{s\in\mathcal{S}}|\sum_{i=1}^n \frac{1}{n}Z_{1,i}^{(3)}| \geq AR_n/2)$, we observe that

$$\begin{aligned}
\left|\frac{1}{n}Z_{1,i}^{(3)}\right| &= \frac{1}{n}|\phi(s)^\top (H_q + \rho W)^{-1}\varphi(T_i)\varepsilon_{1,i,n}| \\
&\leq \frac{2L_n}{n}|\phi(s)^\top (H_q + \rho W)^{-1}\varphi(T_i)| \\
&\leq \frac{2L_n}{n}\|\phi(s)\|_2\|(H_q + \rho W)^{-1}\|\|\varphi(T_i)\|_2 \\
&\leq \frac{c_5 L_n q^\alpha}{n},
\end{aligned}$$

where the last inequality is due to (S12), Lemma 1 and Claim 5. In addition, we have

$$\begin{aligned}
\sum_{i=1}^{n}\mathbb{E}\big(\frac{1}{n}Z_{1,i}^{(3)}\big)^2 &= \frac{1}{n^2}\sum_{i=1}^{n}\mathbb{E}(Z_{1,i}^{(3)})^2 \\
&= \frac{1}{n^2}\sum_{i=1}^{n}\mathbb{E}\varepsilon_{1,i,n}^2\phi(s)^\top(H_q+\rho W)^{-1}\mathbb{E}\{\varphi(T_i)\varphi(T_i)^\top\}(H_q+\rho W)^{-1}\phi(s) \\
&\le \frac{\sigma^2}{n^2}\sum_{i=1}^{n}\|\phi(s)\|_2^2\|(H_q+\rho W)^{-1}\|^2\|\mathbb{E}\{\varphi(T_i)\varphi(T_i)^\top\}\| \\
&\le \frac{c\sigma^2}{n^2}\sum_{i=1}^{n}q^\alpha \\
&\le \frac{c_6q^\alpha}{n},
\end{aligned}$$

where the second inequality is based on (S12), Lemma 1 and Claim 6. Noting that $\mathbb{E}Z_{1,i}^{(3)}=0$, we apply Bernstein's inequality to conclude

$$\begin{aligned}
&\Pr\bigg(\max_{s\in\mathcal{S}}\bigg|\sum_{i=1}^{n}\frac{1}{n}Z_{1,i}^{(3)}\bigg|\ge AR_n/2\bigg) \\
&\le |\mathcal{S}|\max_{s\in\mathcal{S}}\Pr\bigg(\bigg|\sum_{i=1}^{n}\frac{1}{n}Z_{1,i}^{(3)}\bigg|\ge AR_n/2\bigg) \\
&\le cn^{\eta_2}\exp\bigg(-\frac{A^2R_n^2/8}{c_6q^\alpha/n+AR_nL_nc_5q^\alpha/6n}\bigg) \\
&\le cn^{\eta_2}\exp\bigg(-\frac{A^2\log n}{8c_6+(4c_5/3)AL_n\sqrt{q^\alpha\log n/n}}\bigg).
\end{aligned}$$

Under the condition $L_n\le c\sqrt{n/(q^\alpha\log n)}$, $\Pr(\max_{s\in\mathcal{S}}|\frac{1}{n}\sum_{i=1}^{n}Z_{1,i}^{(3)}|\ge AR_n/2)$ decays to zero uniformly over the class $\mathcal{F}$.

To find a bound for the term $\Pr(\max_{s\in\mathcal{S}}|\frac{1}{n}\sum_{i=1}^{n}Z_{2,i}^{(3)}|\ge AR_n/2)$, we first note that $\max_{s\in\mathcal{S}}|\phi(s)^\top(H_q+\rho W)^{-1}\varphi(T_i)|\le\max_{s\in\mathcal{S}}\|\phi(s)\|_2\|(H_q+\rho W)^{-1}\|\|\varphi(T_i)\|_2\le cq^\alpha$ according to (S12), Lemma 1 and Claim 5. By Markov's inequality and Assumption 3, we then deduce that

$$\Pr\bigg(\max_{s\in\mathcal{S}}\bigg|\frac{1}{n}\sum_{i=1}^{n}Z_{2,i}^{(3)}\bigg|\ge AR_n/2\bigg)$$

$$
\begin{aligned}
&\le \Pr\biggl( \max_{s\in\mathcal{S}} \frac{1}{n}\sum_{i=1}^{n} |Z_{2,i}^{(3)}| \ge AR_n/2 \biggr) \\
&= \Pr\biggl( \max_{s\in\mathcal{S}} \frac{1}{n}\sum_{i=1}^{n} |\phi(s)^\top (H_q+\rho W)^{-1}\varphi(T_i)| \cdot |\varepsilon_{2,i,n}| \ge AR_n/2 \biggr) \\
&\le \frac{\mathbb{E}\{\max_{s\in\mathcal{S}} \frac{1}{n}\sum_{i=1}^{n} |\phi(s)^\top (H_q+\rho W)^{-1}\varphi(T_i)||\varepsilon_{2,i,n}|\}}{AR_n/2} \\
&\le \frac{cq^\alpha n^{-1}\sum_{i=1}^{n}\mathbb{E}[|\varepsilon_i| I(|\varepsilon_i|>L_n)]}{AR_n/2} \\
&\le \frac{cq^\alpha}{AR_n}\frac{n^{-1}\sum_{i=1}^{n}\mathbb{E}[|\varepsilon_i|^{2+\xi} I(|\varepsilon_i|>L_n)]}{L_n^{1+\xi}} \\
&\le c/A \to 0 \text{ uniformly over the class } \mathcal{F}
\end{aligned}
$$

by taking $L_n^{1+\xi} \asymp q^\alpha/R_n = \sqrt{q^\alpha n/\log n}$. Note that the previous required condition $L_n \lesssim \sqrt{n/(q^\alpha \log n)}$ is satisfied by this choice due to the assumption $q^\alpha \lesssim (n/\log n)^{\xi/(2+\xi)}$. Together with the decay of $\Pr(\max_{s\in\mathcal{S}} |\frac{1}{n}\sum_{i=1}^{n} Z_{1,i}^{(3)}| \ge AR_n/2)$, the above yields the claim.

**Claim 5.** $\sup_i \|\varphi(T_i)\|_2 \le cq^{\alpha/2}$ *and* $\sup_i \|\Psi_i(u)\|_2 \le c\|u\|_2$ *for* $u \in \mathbb{R}^q$.

The first statement of this claim follows from

$$
\|\varphi(T_i)\|_2^2 = \sum_{j=1}^{q} n^2 n_j^{-2}\phi_j^2(T_i) I(\tau_j \le i) \le c\sum_{j=1}^{q}\phi_j^2(T_i) \le cq^\alpha,
$$

where we note that $(1-c_\circ)n \le n_q \le n_j \le n$ and we utilize (S12). The second statement follows from $\|\Psi_i(u)\|_2 \le nn_q^{-1}\|u\|_2 \le c\|u\|_2$.

**Claim 6.** $\sup_i \|\mathbb{E}\{\varphi(T_i)\varphi(T_i)^\top\}\| \le c$ *and* $\sup_i \|B_i\| \le c$.

For the first statement, for $u \in \mathbb{R}^q$ with $u \ne 0$, we observe

$$
\begin{aligned}
|u^\top \mathbb{E}\{\varphi(T_i)\varphi(T_i)^\top\} u| &= \sum_{j=1}^{q} n^2 n_j^{-2} I(\tau_j \le i)\mathbb{E}\{u_j\phi_j(T_i)\}^2 \\
&\le c\sum_{j=1}^{q}\mathbb{E}\{u_j\phi_j(T_i)\}^2 \\
&\le c\sum_{j=1}^{q}\mathbb{E}_{\mathcal{T}}\{u_j\phi_j(T_i)\}^2
\end{aligned}
$$

$$\leq c\|u\|_2^2, \tag{S18}$$

where the first inequality is due to $(1 - c_\circ)n \leq n_q \leq n_j \leq n$, and the second inequality is based on Assumption 1. This shows that $\sup_i \|\mathbb{E}\{\varphi(T_i)\varphi(T_i)^\top\}\| \leq c$.

For the second statement, noting $\mathbb{E}\big\{\varphi(T_i)\phi(T_i)^\top a - \Psi_i(H_q a)\big\} = 0$, we first observe

$$\begin{aligned} B_i &= \mathbb{E}\{\varphi(T_i)\phi(T_i)^\top a a^\top \phi(T_i)\varphi(T_i)^\top\} - \Psi_i(H_q a)\Psi_i(H_q a)^\top \\ &= \mathbb{E}[\{a^\top \phi(T_i)\}^2\{\varphi(T_i)\varphi(T_i)^\top\}] - \Psi_i(H_q a)\Psi_i(H_q a)^\top. \end{aligned}$$

For the first term, note that $\|a^\top \phi\|_\infty \leq \|m\|_\infty + \|m - a^\top \phi\|_\infty \leq \|m\|_\infty + \kappa_{\phi,\infty}(q) \leq c$. This implies that, for any $u \in \mathbb{R}^q$ with $u \neq 0$, we have

$$|u^\top \mathbb{E}[\{a^\top \phi(T_i)\}^2\{\varphi(T_i)\varphi(T_i)^\top\}]u| \leq c|u^\top \mathbb{E}\{\varphi(T_i)\varphi(T_i)^\top\}u| \leq c\|u\|_2^2,$$

where the last inequality is due to (S18). In other words, $\|\mathbb{E}[\{a^\top \phi(T_i)\}^2\{\varphi(T_i)\varphi(T_i)^\top\}]\| \leq c$. For the second term, for $u \in \mathbb{R}^q$ with $u \neq 0$, we have

$$\begin{aligned} |u^\top \Psi_i(H_q a)\Psi_i(H_q a)^\top u| &= |u^\top \Psi_i(H_q a)|^2 \\ &\leq \|u\|_2^2 \|\Psi_i(H_q a)\|_2^2 \\ &\leq c\|u\|_2^2 \|H_q a\|_2^2 \\ &\leq c\|u\|_2^2 \|H_q\|^2 \|a\|_2^2 \\ &\leq c\|u\|_2^2, \end{aligned}$$

where the second inequality is due to Claim 5 and the last is due to Lemma 1. This shows $\|\Psi_i(H_q a)\Psi_i(H_q a)^\top\| \leq c$. Consequently, $\|B_i\| \leq \|\mathbb{E}[\{a^\top \phi(T_i)\}^2\{\varphi(T_i)\varphi(T_i)^\top\}]\| + \|\Psi_i(H_q a)\Psi_i(H_q a)^\top\| \leq c$.

**Claim 7.** $\|\hat{m} - \acute{m}\|_\infty = O_P^{\mathcal{F}}\big(R_n + \tilde{r}_n + q^{\alpha/2}\tilde{r}_n^2 + q^{\alpha/2}\tilde{r}_n\kappa_{\phi,\infty}(q) + q^{\alpha/2}\kappa_{\psi,\infty}(p)\big)$ *under the conditions* $\kappa_{\psi,\infty}(p) \ll 1$, $\rho \lesssim q^{-\alpha/2-\zeta}$, $p^{2\alpha} \lesssim n/\log n$ *and* $q^{2\alpha} \lesssim n/\log n$, *where* $\tilde{r}_n = r_n + \kappa_{\psi,\infty}(p)$.

We first observe that

$$\begin{aligned} \|\hat{m} - \acute{m}\|_\infty &= \sup_s |\phi(s)^\top \{(\hat{H}_q + \rho W)^{-1} - (H_q + \rho W)^{-1}\}(N_q^{-1} G_q)| \\ &\leq \sup_s |\phi(s)^\top \{(\hat{H}_q + \rho W)^{-1} - (H_q + \rho W)^{-1}\}\mathbb{E}(N_q^{-1} G_q)| \end{aligned}$$

$$
\begin{aligned}
&+\sup_s |\phi(s)^\top \{(\hat{H}_q+\rho W)^{-1}-(H_q+\rho W)^{-1}\}\{N_q^{-1}G_q-\mathbb{E}(N_q^{-1}G_q)\}| \\
&\le \sup_s |\phi(s)^\top \{(\hat{H}_q+\rho W)^{-1}-(H_q+\rho W)^{-1}\}H_q a| \\
&\quad + O_P^{\mathcal{F}}(q^{\alpha/2}\tilde{r}_n\kappa_{\phi,\infty}(q)+\tilde{r}_n q^\alpha/\sqrt{n}),
\end{aligned}
$$

where the last inequality is due to Claim 8 and Lemma 4.

Let $U = H_q + \rho W$, $\hat{U} = \hat{H}_q + \rho W$ and $\Delta = \hat{H}_q - H_q$. Since $\|\Delta\|$ converges to zero in probability uniformly over the class $\mathcal{F}$ according to Lemma 4 and $\|H_q + \rho W\| \asymp 1$ according to Lemma 1 and the condition $\rho q^\zeta \ll 1$ , we can apply Taylor expansion in Theorem 2.2 and Lemma 3.1 of Deadman and Relton (2016) to deduce that $\hat{U}^{-1} - U^{-1} = U^{-1}\Delta U^{-1} + O_P^{\mathcal{F}}(\|\Delta\|^2) = U^{-1}\Delta U^{-1} + O_P^{\mathcal{F}}(\tilde{r}_n^2)$ according to Lemma 4. This yields

$$
\begin{aligned}
&\|\hat{m} - \acute{m}\|_\infty \\
&= \sup_s |\phi(s)^\top\{U^{-1}\Delta U^{-1}\}H_q a| + O_P^{\mathcal{F}}(q^{\alpha/2}\tilde{r}_n^2 + q^{\alpha/2}\tilde{r}_n\kappa_{\phi,\infty}(q) + \tilde{r}_n q^\alpha/\sqrt{n}) \\
&= \sup_s |\phi(s)^\top U^{-1}\Delta a| + O_P^{\mathcal{F}}(q^{\alpha/2+\zeta}\rho\tilde{r}_n + q^{\alpha/2}\tilde{r}_n^2 + q^{\alpha/2}\tilde{r}_n\kappa_{\phi,\infty}(q) + \tilde{r}_n q^\alpha/\sqrt{n}) \\
&= \sup_s |\phi(s)^\top U^{-1}\Delta a| + O_P^{\mathcal{F}}(\tilde{r}_n + q^{\alpha/2}\tilde{r}_n^2 + q^{\alpha/2}\tilde{r}_n\kappa_{\phi,\infty}(q)),
\end{aligned}
$$

where we use the conditions $\rho \lesssim q^{-\alpha/2-\zeta}$ and $q^{2\alpha} \lesssim n/\log n$.

To analyze $\sup_s |\phi(s)^\top U^{-1}\Delta a|$, let $V(s) = \phi(s)\phi(s)^\top$ and $\check{H}_q = \int V(s)\sum_{j=1}^p \theta_j\psi_j(s)ds$. We first observe $\|\check{H}_q - H_q\| \le \kappa_{\psi,\infty}(p)$ and thus $\sup_s |\phi(s)^\top U^{-1}(\check{H}_q - H_q)a| \le cq^{\alpha/2}\kappa_{\psi,\infty}(p)$. To see this, for $v \in \mathbb{R}^q$ with $v \neq 0$, we have

$$
\begin{aligned}
|v^\top(\check{H}_q - H_q)v| &= \left|\int v^\top\phi(s)\phi(s)^\top v\left\{\sum_{j=1}^p \theta_j\psi_j(s) - \sum_{j=1}^\infty \theta_j\psi_j(s)\right\}ds\right| \\
&= \left|\int v^\top\phi(s)\phi(s)^\top v\sum_{j=p+1}^\infty \theta_j\psi_j(s)ds\right| \\
&\le \kappa_{\psi,\infty}(p)\int (v^\top\phi(s))^2 ds \\
&= \kappa_{\psi,\infty}(p)\|v\|_2^2,
\end{aligned}
$$

where the third equality is due to the orthogonality of the basis.

Let $h(s) = \phi(s)^\top U^{-1}(\hat{H}_q - \check{H}_q)a$, and we have

$$\begin{aligned}\|\hat{m} - \acute{m}\|_\infty &\le \|h\|_\infty + \sup_s |\phi(s)^\top U^{-1}(\check{H}_q - H_q)a| + O_P^{\mathcal{F}}(\tilde{r}_n + q^{\alpha/2}\tilde{r}_n^2 + q^{\alpha/2}\tilde{r}_n\kappa_{\phi,\infty}(q)) \\ &= \|h\|_\infty + O_P^{\mathcal{F}}(\tilde{r}_n + q^{\alpha/2}\tilde{r}_n^2 + q^{\alpha/2}\tilde{r}_n\kappa_{\phi,\infty}(q) + q^{\alpha/2}\kappa_{\psi,\infty}(p)).\end{aligned}$$

We complete the proof by analyzing the term $\|h\|_\infty$. By the mean value theorem and the assumption that $\{\phi_j\}_{j=1}^\infty$ is a $(C_\phi, \alpha, \alpha_1)$-basis,

$$\begin{aligned}|h(t) - h(t^*)| &= |\{\phi(t) - \phi(t^*)\}^\top U^{-1}(\hat{H}_q - \check{H}_q)a| \\ &= |(t - t^*)\nabla\phi(t^{**})^\top U^{-1}(\hat{H}_q - \check{H}_q)a| \\ &\le \sqrt{C_\phi}q^{\alpha_1/2}|t - t^*|\|U^{-1}(\hat{H}_q - \check{H}_q)a\|_2 \\ &\le c_7 q^{\alpha_1/2}|t - t^*|\|\hat{H}_q - \check{H}_q\|\end{aligned}$$

where $t^{**}$ is between $t$ and $t^*$. Let $\mathscr{A}_n$ be an event on which $c_7\|\hat{H}_q - \check{H}_q\| \le A$. There exist constants $\eta_1$ and $\eta_2$ which can be chosen such that on $\mathscr{A}_n$, for all sufficiently large $A$,

$$c_7 q^{\alpha_1}|t - t^*|\|\hat{H}_q - \check{H}_q\| \le A\sqrt{\frac{q^\alpha \log n}{n}} := AR_n$$

whenever $|t - t^*| \le \eta_1 n^{-\eta_2}$; this is feasible due to the condition $q^\alpha \le C_*(n/\log n)^{1/2}$.

Let $\mathcal{S}$ be a smallest subset of $\mathcal{T}$ satisfying that, for each $t \in \mathcal{T}$, there exists an $s \in \mathcal{S}$ such that $|s - t| \le \eta_1 n^{-\eta_2}$. If $s_n(t)$ denotes the $s \in \mathcal{S}$ that is closest to $t$, then on the event $\mathscr{A}_n$, we have

$$\sup_{t\in\mathcal{T}} |h(t) - h(s_n(t))| \le AR_n. \tag{S19}$$

Let $\overline{\mathscr{A}}_n$ denote the complement of $\mathscr{A}_n$. According to the simple fact $\Pr(E_1) \le \Pr(E_1 \cap E_2) + \Pr(\overline{E}_2)$ for any two events $E_1$ and $E_2$, we deduce that

$$\begin{aligned}\Pr\big(\|h\|_\infty \ge 2AR_n\big) &\le \Pr\big(\{\|h\|_\infty \ge 2AR_n\} \cap \mathscr{A}_n\big) + \Pr(\overline{\mathscr{A}}_n) \\ &\le \Pr\big(\{\sup_{t\in\mathcal{T}} |h(t) - h(s_n(t))| \ge AR_n\} \cap \mathscr{A}_n\big) \\ &\quad + \Pr\big(\{\max_{s\in\mathcal{S}} |h(s)| \ge AR_n\} \cap \mathscr{A}_n\big) + \Pr(\overline{\mathscr{A}}_n) \\ &= \Pr\big(\{\max_{s\in\mathcal{S}} |h(s)| \ge AR_n\} \cap \mathscr{A}_n\big) + \Pr(\overline{\mathscr{A}}_n) \\ &\le \Pr\big(\max_{s\in\mathcal{S}} |h(s)| \ge AR_n\big) \end{aligned} \tag{S20}$$

$$+\Pr(\overline{\mathscr{A}}_n),$$

where the first equality is due to (S19).

We then observe that $\Pr(\overline{\mathscr{A}}_n)$ decays to zero uniformly over the class $\mathcal{F}$ since $\|\hat{H}_q - \check{H}_q\| = O_P^{\mathcal{F}}(r_n)$ and $r_n \lesssim 1$. To see this, for $u = \mathbb{R}^q$ with $u \neq 0$, we observe that

$$\begin{aligned}
|u^\top(\hat{H}_q - \check{H}_q)u| &= \left|u^\top \int V(s)u(\hat{f}(s) - \theta^\top\psi(s))\,ds\right| \\
&= \left|\int (u^\top\phi(s))^2(\hat{f}(s) - \theta^\top\psi(s))\,ds\right| \\
&\leq \sup_s |\hat{f}(s) - \theta^\top\psi(s)| \int (u^\top\phi(s))^2\,ds \\
&= \|u\|_2^2 \sup_s |\hat{f}(s) - \theta^\top\psi(s)| \\
&= O_P^{\mathcal{F}}(r_n)\|u\|_2^2
\end{aligned}$$

according to the proof of Proposition 1.

It remains to establish a bound for (S20). Define $\varrho_i(s) = (\psi_1(s)I(i \geq \tau_1), \ldots, \psi_p(s)I(i \geq \tau_p))^\top$ and $\vartheta_i = (\theta_1 I(i \geq \tau_1), \ldots, \theta_p I(i \geq \tau_p))^\top$. Let $\Delta_i = n\int V(s)\sum_{j=1}^p n_j^{-1}\{\psi_j(T_i) - \theta_j\}I(i \geq \tau_j)\psi_j(s)ds$, and $Z_i = \phi(s)^\top U^{-1}\Delta_i a$. Then $\mathbb{E}Z_i = 0$ and $h(s) = n^{-1}\sum_{i=1}^n Z_i$. In addition, for $u \in \mathbb{R}^q$ with $u \neq 0$, we observe that

$$\begin{aligned}
|u^\top\Delta_i u| &= \left|\int (u^\top\phi(s))^2\psi(s)^\top\{\varrho_i(T_i) - \vartheta_i\}ds\right| \\
&\leq \int (u^\top\phi(s))^2\|\psi(s)\|_2\|\varrho_i(T_i) - \vartheta_i\|_2 ds \\
&\leq cp^\alpha \int (u^\top\phi(s))^2 ds \\
&\leq cp^\alpha\|u\|_2^2.
\end{aligned}$$

This shows that $\|\Delta_i\| \leq cp^\alpha$, based on which we further deduce that

$$\left|\frac{1}{n}Z_i\right| = \left|\frac{1}{n}\phi(s)^\top U^{-1}\Delta_i a\right| \leq \frac{1}{n}\|\phi(s)\|_2\|U^{-1}\|\|\Delta_i a\|_2 \leq cn^{-1}q^{\alpha/2}\|\Delta_i\|\|a\|_2 \leq c_8 p^\alpha q^{\alpha/2}/n.$$

Moreover, we have

$$\begin{aligned}
\sum_{i=1}^{n} \mathbb{E}\{\frac{1}{n}Z_i\}^2 &= n^{-2}\sum_{i=1}^{n} \mathbb{E}[\{\phi(s)^\top U^{-1}\}\Delta_i a a^\top \Delta_i \{\phi(s)^\top U^{-1}\}^\top] \\
&\le n^{-2}\sum_{i=1}^{n} \|\phi(s)^\top U^{-1}\|^2 \left\| \int V(s)a\psi(s)^\top \Gamma_i \psi(t) a^\top V(t) ds dt \right\| \\
&\le n^{-2}\sum_{i=1}^{n} c\|\phi(s)\|_2^2 \|U^{-1}\|^2 \\
&\le n^{-2}\sum_{i=1}^{n} c q^{\alpha} \\
&\le c_9 q^{\alpha}/n,
\end{aligned}$$

where $\Gamma_i = \mathbb{E}[\{\varrho_i(T_i) - \vartheta_i\}\{\varrho_i(T_i) - \vartheta_i\}^\top]$ and the second inequality is based on

$$\sup_{0\le i\le n} \left\| \int V(s)a\psi(s)^\top \Gamma_i \psi(t) a^\top V(t) ds dt \right\| \le c \tag{S21}$$

that we establish now. First, for $u \in \mathbb{R}^q$ with $u \neq 0$, we have

$$\begin{aligned}
|u^\top \Gamma_i u| &= |u^\top \mathbb{E}[\{\varrho_i(T_i) - \vartheta_i\}\{\varrho_i(T_i) - \vartheta_i\}^\top] u| \\
&\le \mathbb{E}|u^\top \{\varrho_i(T_i) - \vartheta_i\}|^2 \\
&= \mathbb{E}\sum_{j=1}^{p} \{u_j(\psi_j(T_i) - \theta_j) I(i \ge \tau_j)\}^2 \\
&\le 2c\mathbb{E}_{\mathcal{T}} \sum_{j=1}^{p} \{u_j^2 \psi_j^2(T_i) + (u_j\theta_j)^2\} \\
&\le c_{10}\|u\|_2^2,
\end{aligned}$$

where the third inequality is due to $\|\theta\|_2^2 \le c$. This shows that $\sup_{0\le i\le n} \|\Gamma_i\| \le c_{10}$. Consequently, for $u \in \mathbb{R}^q$ with $u \neq 0$, we deduce

$$\begin{aligned}
\left| \int u^\top V(s)a\psi(s)^\top \Gamma_i \psi(t) a^\top V(t) u ds dt \right| &= \left| \left[\int u^\top V(s) a\psi(s)^\top ds\right] \Gamma_i \left[\int \psi(t) a^\top V(t) u dt\right] \right| \\
&\le c_{10} \left\| \int u^\top \phi(t)\phi(t)^\top a\psi(t) dt \right\|_2^2 .
\end{aligned}$$

Expand the function $u^\top \phi\phi^\top a$ with respect to $\{\psi_j\}_{j=1}^\infty$, that is, $u^\top \phi(t)\phi(t)^\top a = \sum_{j=1}^\infty v_j \psi_j(t)$ for real coefficients $v_1, \ldots$. Then the term $\left\| \int u^\top \phi(t)\phi(t)^\top a \psi(t) dt \right\|_2^2$ is exactly $\|v\|_2^2$ with $v = (v_1, \ldots, v_p)^\top$. We further deduce

$$\left\| \int u^\top \phi(t)\phi(t)^\top a \psi(t) dt \right\|_2^2 = \|v\|_2^2 \le \|u^\top \phi\phi^\top a\|_{L^2}^2 \le \|u^\top \phi\|_{L^2}^2 \|\phi^\top a\|_\infty^2 \le c\|u\|_2^2,$$

where we note that $\|\phi^\top a\|_\infty \le \|m\|_\infty + \|m - \phi^\top a\|_\infty \le M + \kappa_{\phi,\infty}(q) \le c$. This finally proves (S21).

Now according to Bernstein's inequality,

$$\begin{aligned}
\Pr(|h(s)| \ge AR_n) &= \Pr\left( \left| \frac{1}{n} \sum_{i=1}^n Z_i \right| \ge AR_n \right) \\
&\le \exp\left( - \frac{A^2 R_n^2}{c_9 q^\alpha / n + c_8 p^\alpha q^{\alpha/2} AR_n / 3n} \right) \\
&= \exp\left( - \frac{A^2 \log n}{c_9 + c_8 A p^\alpha \sqrt{\log n} / (3\sqrt{n})} \right) \\
&\le \exp(-cA \log n) = n^{-cA},
\end{aligned}$$

where the last inequality holds due to the condition $p^{2\alpha} \lesssim n/\log n$. The above inequality implies that

$$\Pr\left( \max_{s \in \mathcal{S}} |h(s)| \ge AR_n \right) \le |\mathcal{S}| n^{-cA} \le c n^{\eta_2 - cA} \to 0$$

uniformly over the class $\mathcal{F}$. This gives the desired bound for (S20) and concludes the proof of the claim.

**Claim 8.** *$\sup_{F \in \mathcal{F}} \|\mathbb{E}_F(N_q^{-1} G_q) - H_q a\|_2^2 \le c(1 + q^\alpha/n)\kappa_{\phi,\infty}^2(q)$ and $\sup_{F \in \mathcal{F}} \mathbb{E}_F \|N_q^{-1} G_q - \mathbb{E}_F(N_q^{-1} G_q)\|_2^2 \le c q^\alpha / n$.*

To see these, let $\hat{\Phi}$ be an $n \times q$ matrix with elements $\hat{\Phi}_{ij} = n_j^{-1} \phi_j(T_i) I(i \ge \tau_j)$. Define $Y = (Y_1, Y_2, \ldots, Y_n)^\top$, $\tilde{Y} = (m(T_1), m(T_2), \ldots, m(T_n))^\top$, and $\varepsilon = (\varepsilon_1, \varepsilon_2, \ldots, \varepsilon_n)^\top$. Then $\mathbb{E}_F(N_q^{-1} G_q) = \mathbb{E}(\hat{\Phi}^\top Y) = \mathbb{E}\{\hat{\Phi}^\top (\tilde{Y} + \varepsilon)\} = \mathbb{E}(\hat{\Phi}^\top \tilde{Y})$. Recall that $\Phi$ is the $n \times q$ matrix with elements $\Phi_{ij} = \phi_j(T_i)$. Define $\bar{m} = m - a^\top \phi$. Then we have $\mathbb{E}_F(N_q^{-1} G_q) = \mathbb{E}\{\hat{\Phi}^\top (\Phi a +$

$\tilde{Y} - \Phi a)\} = \mathbb{E}\{\hat{\Phi}^\top \Phi a\} + \mathbb{E}\{\hat{\Phi}^\top(\tilde{Y} - \Phi a)\} = H_q a + \mathbb{E}\{\hat{\Phi}^\top(\tilde{Y} - \Phi a)\}$ and

$$
\begin{aligned}
\mathbb{E}\|\hat{\Phi}^\top(\tilde{Y} - \Phi a)\|_2^2 &= \mathbb{E}_F \sum_{j=1}^{q} \left\{ \sum_{i=1}^{n} n_j^{-1} \phi_j(T_i)(m(T_i) - a^\top \phi(T_i)) I(i \geq \tau_j) \right\}^2 \\
&= \sum_{j=1}^{q} \mathbb{E}_F \left\{ \sum_{i=1}^{n} n_j^{-1} \bar{m}(T_i) \phi_j(T_i) I(i \geq \tau_j) \right\}^2 \\
&= \sum_{j=1}^{q} \sum_{i \neq k} n_j^{-2} [\mathbb{E}_F\{\bar{m}(T)\phi_j(T)\}]^2 I(\tau_j \leq i, \tau_j \leq k) \\
&\quad + \sum_{j=1}^{q} \sum_{i=1}^{n} n_j^{-2} \mathbb{E}_F\{\bar{m}(T)\phi_j(T)\}^2 I(\tau_j \leq i) \\
&\leq c\|\mathbb{E}_F\{\bar{m}(T)\phi(T)\}\|_2^2 + cn^{-1}\|\bar{m}\|_\infty^2 \mathbb{E}_F\|\phi(T)\|_2^2 \\
&\leq c\|\bar{m}\|_{L^2}^2 + cq^\alpha n^{-1}\|\bar{m}\|_\infty^2 \\
&\leq c(1 + q^\alpha/n)\kappa_{\phi,\infty}^2(q),
\end{aligned}
$$

where we utilize Lemma 2 to obtain the second inequality and $\|\bar{m}\|_{L^2} \leq c\|\bar{m}\|_\infty$ to derive the last inequality. This verifies the first statement.

With the notation $\mathbb{E}_F(N_q^{-1}G_q) = (u_1, \ldots, u_q)^\top$, the second statement is verified by

$$
\begin{aligned}
\mathbb{E}_F\|N_q^{-1}G_q - \mathbb{E}_F(N_q^{-1}G_q)\|_2^2 &= \mathbb{E}_F \sum_{j=1}^{q} \left\{ \frac{1}{n_j} \sum_{i=\tau_j}^{n} [\phi_j(T_i)Y_i - u_j] \right\}^2 \\
&= \sum_{j=1}^{q} n_j^{-2} \sum_{i=\tau_j}^{n} \mathrm{var}(\phi_j(T_i)Y_i) \\
&\leq \frac{c}{n^2} \sum_{j=1}^{q} \sum_{i=1}^{n} \mathbb{E}\{\phi_j(T_i)Y_i\}^2 \\
&= \frac{c}{n^2} \sum_{i=1}^{n} \mathbb{E}\left\{ Y_i^2 \sum_{j=1}^{q} \phi_j^2(T_i) \right\} \\
&\leq \frac{cq^\alpha}{n^2} \sum_{i=1}^{n} \mathbb{E}(Y_i^2) \\
&\leq cq^\alpha/n,
\end{aligned}
$$

where the first inequality is partially due to $n_j \geq n_q \geq (1 - c_\circ)n$ for all $1 \leq j \leq q$, the

second inequality is based on (S12), and the last is due to $\mathbb{E}(Y_i^2) \le c$ for all $i = 1, \ldots, n$. $\square$

## S3 Proof of Theorem 2

*Proof of Theorem 2.* By the assumed conditions, there exists a constant $C_* > 0$ such that $p^\alpha \le C_* n/\log n$, $\kappa_{\psi,\infty}(p) \le C_*$, $\kappa_{\phi,\infty}(q) \le C_*$, $\rho q^\zeta \le C_* R_n$ and $q^\alpha \le C_* n$.

We first observe that

$$\|\hat{m} - m\|_{L^2} \le \|\hat{a} - a\|_2 + \kappa_{\phi,2}(q)$$

and

$$\begin{aligned} \|\hat{a} - a\|_2 =& \|(\hat{H}_q + \rho W)^{-1}(N_q^{-1} G_q) - a\|_2 \\ \le& c\|[(\hat{H}_q + \rho W)^{-1} - (H_q + \rho W)^{-1}](N_q^{-1} G_q)\|_2 \\ &+ c\|[(H_q + \rho W)^{-1} - H_q^{-1}](N_q^{-1} G_q)\|_2 \\ &+ c\|H_q^{-1}(N_q^{-1} G_q) - a\|_2 \\ \equiv& c(\mathrm{I} + \mathrm{II} + \mathrm{III}). \end{aligned}$$

The theorem follows from the bounds for these terms that are addressed separately below.

*Term* I. This term is zero when $f$ is known. Otherwise, let $\Delta = \hat{H}_q - H_q$, $\hat{U} = \hat{H}_q + \rho W$ and $U = H_q + \rho W$. Let $I_q$ denote the $q \times q$ identity matrix. Using the fact that $\hat{U}^{-1} - U^{-1} = -(I_q + U^{-1}\Delta)^{-1} U^{-1} \Delta U^{-1}$, we deduce

$$\begin{aligned} \mathrm{I} &\le \|(\hat{H}_q + \rho W)^{-1} - (H_q + \rho W)^{-1}\| \cdot \|N_q^{-1} G_q\|_2 \\ &= \|(I_q + U^{-1}\Delta)^{-1} U^{-1} \Delta U^{-1}\| \cdot \|N_q^{-1} G_q\|_2 \\ &\le c\|(I_q + U^{-1}\Delta)^{-1}\| \cdot \|\Delta\| \cdot \|N_q^{-1} G_q\|_2. \end{aligned}$$

Then Lemmas 3 and 4 imply that

$$\lim_{A\to\infty} \limsup_{n\to\infty} \sup_{F\in\mathcal{F}} \Pr_F(\mathrm{I} \ge A(r_n + \kappa_{\psi,\infty}(p))) = 0$$

given $q^\alpha \lesssim n$.

*Term* II. Note that $(H_q + \rho W)^{-1} - H_q^{-1} = -(I_q + \rho H_q^{-1} W)^{-1} H_q^{-1} (\rho W) H_q^{-1}$. We then have

$$\mathrm{II} \le \|(I_q + \rho H_q^{-1} W)^{-1}\| \cdot \|H_q^{-1}\|^2 \cdot \|\rho W\| \cdot \|N_q^{-1} G_q\|_2 \le c\rho q^{\zeta} \|N_q^{-1} G_q\|_2.$$

Thus, according to Lemma 3 and the assumption $q^{\alpha} \lesssim n$,

$$\sup_{F\in\mathcal{F}} \mathbb{E}_F(\mathrm{II}) \le c\rho q^{\zeta} \le cR_n. \tag{S22}$$

*Term* III. Recall that $\Phi$ is the $n \times q$ matrix of elements $\phi_j(T_i)$, i.e., the design matrix from the full data up to the current time $n$. We first observe

$$\begin{aligned}
\mathrm{III} &\le \|H_q^{-1} N_q^{-1} G_q - n^{-1} H_q^{-1} \Phi^{\top} Y\|_2 + \|n^{-1} H_q^{-1} \Phi^{\top} Y - a\|_2 \\
&\le \|H_q^{-1}\| \cdot \|N_q^{-1} G_q - n^{-1} \Phi^{\top} Y\|_2 + \|n^{-1} H_q^{-1} \Phi^{\top} Y - a\|_2 \\
&\le c\|N_q^{-1} G_q - n^{-1} \Phi^{\top} Y\|_2 + \|n^{-1} H_q^{-1} \Phi^{\top} Y - a\|_2,
\end{aligned}$$

where the last inequality is due to Lemma 1. The first term in the above is addressed in Claim 9. For the second term, with $\tilde{Y} = (m(T_1), \ldots, m(T_n))^{\top}$ and $\varepsilon = (\varepsilon_1, \ldots, \varepsilon_n)^{\top}$, we have

$$\begin{aligned}
\|n^{-1} H_q^{-1} \Phi^{\top} Y - a\|_2 &= \|n^{-1} H_q^{-1} \Phi^{\top} (\Phi a + (\tilde{Y} - \Phi a) + \varepsilon) - a\|_2 \\
&\le \|n^{-1} H_q^{-1} \Phi^{\top} \Phi a - a\|_2 + \|n^{-1} H_q^{-1} \Phi^{\top} (\tilde{Y} - \Phi a)\|_2 + \|n^{-1} H_q^{-1} \Phi^{\top} \varepsilon\|_2 \\
&\le \|n^{-1} H_q^{-1} \Phi^{\top} \Phi a - a\|_2 + \|n^{-1} H_q^{-1} \Phi^{\top} (\tilde{Y} - \Phi a)\|_2 + c\|n^{-1} \Phi^{\top} \varepsilon\|_2,
\end{aligned}$$

where we use Lemma 1 to obtain the last inequality. According to Claims 10, 11 and 12, along with Claim 9 for the first term, we conclude that

$$\sup_{F\in\mathcal{F}} \mathbb{E}_F(\mathrm{III}) \le c\{R_n + \kappa_{\phi,2}(q)\}. \tag{S23}$$

Now we state and establish the claims referenced in the above arguments to complete the proof of the theorem. Note that all constants $c, c_1, \ldots$ below are independent of $F \in \mathcal{F}$, and thus to prove the claims involving a uniform bound over *all* $F \in \mathcal{F}$ it is sufficient to prove them for *any* $F$.

**Claim 9.** $\sup_{F\in\mathcal{F}} \mathbb{E}_F \|N_q^{-1} G_q - n^{-1} \Phi^{\top} Y\|_2^2 \le c q^{\alpha}/n$.

Let $u = (u_1, \ldots, u_q)^\top$ with $u_j = \mathbb{E}_F\{\phi_j(T)Y\}$ for $j = 1, \ldots, q$. We first observe

$$\begin{aligned}
\mathbb{E}_F\|N_q^{-1}G_q - u\|_2^2 &= \mathbb{E}_F \sum_{j=1}^{q} \left\{ \frac{1}{n_j} \sum_{i=\tau_j}^{n} \phi_j(T_i)Y_i - u_j \right\}^2 \\
&= \sum_{j=1}^{q} n_j^{-2} \sum_{i=\tau_j}^{n} \mathrm{var}(\phi_j(T_i)Y_i) \\
&\le \frac{c}{n^2} \sum_{j=1}^{q} \sum_{i=1}^{n} \mathbb{E}_F\{\phi_j(T_i)Y_i\}^2 \\
&= \frac{c}{n^2} \sum_{i=1}^{n} \mathbb{E}_F \left\{ Y_i^2 \sum_{j=1}^{q} \phi_j^2(T_i) \right\} \\
&\le \frac{cq^\alpha}{n^2} \sum_{i=1}^{n} \mathbb{E}_F Y_i^2 \\
&\le cq^\alpha/n,
\end{aligned}$$

where the first inequality is partially due to $n_j \ge n_q \ge (1-c_\circ)n$ for all $1 \le j \le q$, the second inequality is based on (S12), and the last is due to $\mathbb{E}(Y_i^2) \le c$ for all $i = 1, \ldots, n$. A similar argument shows that $\mathbb{E}_F\|n^{-1}\Phi^\top Y - u\|_2^2 \le cq^\alpha/n$. Consequently, $\mathbb{E}_F\|N_q^{-1}G_q - n^{-1}\Phi^\top Y\|_2^2 \le 2\mathbb{E}_F\|N_q^{-1}G_q - u\|_2^2 + 2\mathbb{E}_F\|n^{-1}\Phi^\top Y - u\|_2^2 \le cq^\alpha/n$.

**Claim 10.** $\sup_{F\in\mathcal{F}} \mathbb{E}_F\|n^{-1}H_q^{-1}\Phi^\top(\tilde{Y} - \Phi a)\|_2^2 \le c(1 + q^\alpha/n)\kappa_{\phi,2}^2(q)$.

The claim follows from the following observation:

$$\begin{aligned}
\mathbb{E}_F\|n^{-1}H_q^{-1}\Phi^\top(\tilde{Y} - \Phi a)\|_2^2 &= \frac{1}{n^2}\mathbb{E}_F \left\| \sum_{i=1}^{n} H_q^{-1}\phi(T_i)\bar{m}(T_i) \right\|_2^2 \\
&= \frac{1}{n^2}\mathbb{E}_F \left\{ \sum_{i,j=1}^{n} \bar{m}(T_i)\phi(T_i)^\top H_q^{-1}H_q^{-1}\phi(T_j)\bar{m}(T_j) \right\} \\
&= \frac{n^2 - n}{n^2}\mathbb{E}_F\{\bar{m}(T)\phi(T)^\top\}H_q^{-1}H_q^{-1}\mathbb{E}_F\{\phi(T)\bar{m}(T)\} \\
&\quad + \frac{1}{n}\mathbb{E}_F\{\bar{m}(T)\phi(T)^\top H_q^{-1}H_q^{-1}\phi(T)\bar{m}(T)\} \\
&\le \|\mathbb{E}_F\{\bar{m}(T)\phi(T)\}\|_2^2\|H_q^{-1}\|^2 + \frac{1}{n}\mathbb{E}_F\{|\bar{m}(T)|^2\|\phi(T)\|_2^2\|H_q^{-1}\|^2\} \\
&\le c\|\bar{m}\|_{L^2}^2 + \frac{cq^\alpha}{n}\mathbb{E}_F|\bar{m}(T)|^2
\end{aligned}$$

$$
\begin{aligned}
&\leq c(1+q^\alpha/n)\|\bar{m}\|_{L^2}^2 \\
&\leq c(1+q^\alpha/n)\kappa_{\phi,2}^2(q)
\end{aligned}
$$

where we use Lemma 1, Lemma 2 and (S12) to obtain the second inequality, and use Assumption 1 for the third inequality.

**Claim 11.** $\sup_{F\in\mathcal{F}} \mathbb{E}_F\|n^{-1}\Phi^\top\varepsilon\|_2^2 \leq cq^\alpha/n$.

The claim follows from the observation

$$
\begin{aligned}
\mathbb{E}_F\|n^{-1}\Phi^\top\varepsilon\|_2^2 &= \frac{1}{n^2}\mathbb{E}_F\sum_{j=1}^q\Big\{\sum_{i=1}^n\phi_j(T_i)\varepsilon_i\Big\}^2 \\
&= \frac{1}{n^2}\sum_{j=1}^q\sum_{i=1}^n\mathbb{E}_F\{\phi_j^2(T_i)\varepsilon_i^2\} \\
&\leq \frac{c\sigma^2}{n}\sum_{j=1}^q\mathbb{E}_F\phi_j^2(T) \\
&\leq \frac{cq^\alpha}{n},
\end{aligned}
$$

where the last inequality is based on (S12).

**Claim 12.** $\sup_{F\in\mathcal{F}} \mathbb{E}_F\|n^{-1}H_q^{-1}\Phi^\top\Phi a - a\|_2^2 \leq cq^\alpha/n$.

To show this, we first note that $n^{-1}\Phi^\top\Phi a = n^{-1}\sum_{i=1}^n\phi(T_i)\phi(T_i)^\top a$. In addition, $\mathbb{E}_F\{H_q^{-1}\phi(T_i)\phi(T_i)^\top a - a\} = 0$. Then,

$$
\begin{aligned}
\mathbb{E}_F\|n^{-1}H_q^{-1}\Phi^\top\Phi a - a\|_2^2 &= \mathbb{E}_F\left[\frac{1}{n^2}\sum_{i,j=1}^n\{H_q^{-1}\phi(T_i)\phi(T_i)^\top a - a\}^\top\{H_q^{-1}\phi(T_j)\phi(T_j)^\top a - a\}\right] \\
&= n^{-1}\mathbb{E}_F[\{H_q^{-1}\phi(T)\phi(T)^\top a - a\}^\top\{H_q^{-1}\phi(T)\phi(T)^\top a - a\}] \\
&= n^{-1}\mathbb{E}_F\{a^\top\phi(T)\phi(T)^\top H_q^{-1}H_q^{-1}\phi(T)\phi(T)^\top a\} - n^{-1}a^\top a \\
&\leq n^{-1}\mathbb{E}_F|a^\top\phi(T)\phi(T)^\top H_q^{-1}H_q^{-1}\phi(T)\phi(T)^\top a| \\
&\leq n^{-1}\|\phi^\top a\|_\infty^2\|H_q^{-1}\|^2\mathbb{E}_F\{\|\phi(T)\|_2^2\} \\
&\leq cq^\alpha/n,
\end{aligned}
$$

where in the last inequality we use Lemma 1, the fact $\|\phi^\top a\|_\infty \leq \|m\|_\infty + \|m-\phi^\top a\|_\infty \leq M + \kappa_{\phi,\infty}(q) \leq c$, and $\mathbb{E}_F\|\phi(T)\|_2^2 \leq \sup_t\|\phi(t)\|_2^2 \leq C_\phi q^\alpha$ since $\{\phi_j\}_{j=1}^\infty$ is assumed to be a

$(C_\phi, \alpha)$-basis.

□

# S4 Technical Lemmas

**Lemma 1.** *It holds that* $\inf_{t\in\mathcal{T}} |f(t)| \le \lambda_{\min}(H_q) \le \lambda_{\max}(H_q) \le \|f\|_\infty$ *for all* $q$*. In addition, if* $\rho \ge 0$ *and* $W$ *is positive semi-definite, then* $\|(H_q + \rho W)^{-1}\| \le (\inf_{t\in\mathcal{T}} |f(t)|)^{-1}$ *for all* $q$*.*

*Proof.* To prove the lemma, for any $v \in \mathbb{R}^q$ with $v \neq 0$, we have

$$\begin{aligned} v^\top H_q v &= \int v^\top \phi(t)\phi(t)^\top v f(t)dt \\ &= \int |v^\top \phi(t)|_2^2 f(t)dt \\ &\le \|f\|_\infty \int |v^\top \phi(t)|_2^2 dt \\ &= \|f\|_\infty \|v\|_2^2. \end{aligned}$$

This shows that $\lambda_{\max}(H_q) \le \|f\|_\infty$. A similar argument leads to $\lambda_{\min}(H_q) \ge \inf_{t\in\mathcal{T}} |f(t)|$. Also, $\|(H_q + \rho W)^{-1}\| \le \lambda_{\min}(H_q + \rho W)^{-1} \le \lambda_{\min}(H_q)^{-1} \le (\inf_{t\in\mathcal{T}} |f(t)|)^{-1}$ since $\rho \ge 0$ and $W$ is positive semi-definite. □

**Lemma 2.** *If* $Q$ *is the square root of* $H_q^{-1}$*, then* $\|\mathbb{E}_f\{Q\phi(T)g(T)\}\|_2^2 \le \|f\|_\infty \|g\|_{L^2}^2$*. Consequently,* $\|\mathbb{E}_f\{\phi(T)g(T)\}\|_2^2 \le (\inf_{t\in\mathcal{T}} |f(t)|)^{-1} \|f\|_\infty \|g\|_{L^2}^2$*.*

*Proof.* Note that the elements of $Q\phi$ are orthonormal functions in the space $L^2(\mathcal{T}, f) = \{h : \int_\mathcal{T} h^2(t)f(t)dt < \infty\}$ endowed with the inner product $\int_\mathcal{T} h_1(t)h_2(t)f(t)dt$ for $h_1, h_2 \in L^2(\mathcal{T}, f)$. Then $\mathbb{E}_f\{Q\phi(T)g(T)\}$ contains precisely the $q$ generalized Fourier coefficients of $g$ with respect to the element of $Q\phi$. Consequently, $\|\mathbb{E}_f\{Q\phi(T)g(T)\}\|_2^2 \le \|g\|_{L^2(\mathcal{T},f)}^2 \le \|f\|_\infty \|g\|_{L^2}^2$. Also, $\|\mathbb{E}_f\{\phi(T)g(T)\}\|_2^2 = \|Q^{-1}\mathbb{E}_f\{Q\phi(T)g(T)\}\|_2^2 \le \|Q^{-1}\|^2 \|f\|_\infty \|g\|_{L^2}^2 \le (\inf_{t\in\mathcal{T}} |f(t)|)^{-1} \|f\|_\infty \|g\|_{L^2}^2$. □

**Lemma 3.** *If* $\sigma^2 < \infty$ *and* $\{\phi_j\}_{j=1}^\infty$ *is a* $(C_\phi, \alpha)$*-basis, then* $\sup_{F\in\mathcal{F}} \mathbb{E}_F \|N_q^{-1} G_q\|_2^2 \le c(1 + q^\alpha/n)$ *for a constant* $c > 0$ *depending only on* $\mathcal{T}$*,* $M$*,* $C_{f,1}$*,* $C_{f,2}$*,* $c_\circ$*,* $C_\phi$ *and* $\sigma^2$*.*

*Proof.* The lemma follows from the observation

$$\begin{aligned}
\mathbb{E}_F\|N_q^{-1}G_q\|_2^2 &= \mathbb{E}_F\sum_{j=1}^q \frac{1}{n_j^2}\Big\{\sum_{i=\tau_j}^n \phi_j(T_i)Y_i\Big\}^2 \\
&= \mathbb{E}_F\sum_{j=1}^q \frac{1}{n_j^2}\Big\{\sum_{i=\tau_j}^n \phi_j(T_i)m(T_i)\Big\}^2 + \sum_{j=1}^q \frac{1}{n_j^2}\sum_{i=\tau_j}^n \mathbb{E}_F\{\phi_j^2(T_i)\varepsilon_i^2\} \\
&\le c\sum_{j=1}^q \frac{1}{n_j^2}\{n_j^2[\mathbb{E}_F\{\phi_j(T)m(T)\}]^2 + n_j\mathbb{E}_F\phi_j^2(T)m^2(T)\} + \sigma^2\sum_{j=1}^q \frac{\mathbb{E}_F\phi_j^2(T)}{n_j} \\
&\le c\|\mathbb{E}_f\{\phi(T)m(T)\}\|_2^2 + c\|m\|_\infty^2\sum_{j=1}^q \frac{\mathbb{E}_F\phi_j^2(T)}{n_j} + \sigma^2\sum_{j=1}^q \frac{\mathbb{E}_F\phi_j^2(T)}{n_j} \\
&\le c\|m\|_{L^2}^2 + \frac{c\|m\|_\infty^2}{n}\sum_{j=1}^q \mathbb{E}_F\phi_j^2(T) + \frac{c}{n}\sum_{j=1}^q \mathbb{E}_F\phi_j^2(T) \\
&\le c\|m\|_{L^2}^2 + \frac{cq^\alpha}{n} + \frac{cq^\alpha}{n} \\
&\le c(1+q^\alpha/n),
\end{aligned}$$

where we use $\mathbb{E}_F\{\phi_j(T_1)\phi_j(T_2)m(T_1)m(T_2)\} = \mathbb{E}_F\{\phi_j(T_1)m(T_1)\}\mathbb{E}_F\{\phi_j(T_2)m(T_2)\}$ for any independent $T_1$ and $T_2$ in the first equality, the third inequality is due to Lemma 2 and $n \ge n_j \ge n_q \ge (1-c_\circ)n$, and we use (S12) in the fourth inequality. □

**Lemma 4.** *Under Assumption 4, for any $\ell > 0$, $\sup_{f\in\mathcal{D}(\gamma,\chi,M)}\mathbb{E}\|\hat{H}_q - H_q\|^\ell \lesssim \big(r_n + \kappa_{\psi,\infty}(p)\big)^\ell$ with $r_n = p^{\alpha/2}(n/\log n)^{-1/2}$. In addition, if $\rho \ge 0$ and $W$ is positive semi-definite, then*

$$\lim_{A\to\infty}\limsup_{n\to\infty}\sup_{F\in\mathcal{F}}\Pr_F\big(\|(\hat{H}_q+\rho W)^{-1} - (H_q+\rho W)^{-1}\| \ge A\{r_n + \kappa_{\psi,\infty}(p)\}\big) = 0, \quad \text{(S24)}$$

*provided $r_n + \kappa_{\psi,\infty}(p) \ll 1$.*

*Proof.* Let $\Delta = \hat{H}_q - H_q$ and note that $\Delta$ is symmetric. For any $\ell > 0$,

$$\begin{aligned}
\sup_{f\in\mathcal{D}(\gamma,\chi,M)}\mathbb{E}_f\|\Delta\|^\ell &= \sup_{f\in\mathcal{D}(\gamma,\chi,M)}\mathbb{E}_f\Big\{\sup_{\|v\|_2=1}|v^\top\Delta v|\Big\}^\ell \\
&= \sup_{f\in\mathcal{D}(\gamma,\chi,M)}\mathbb{E}_f\Big\{\sup_{\|v\|_2=1}\Big|\int_{\mathcal{T}}(v^\top\phi(t))^2(\hat{f}(t)-f(t))dt\Big|\Big\}^\ell
\end{aligned}$$

$$
\begin{aligned}
&\leq \sup_{f\in\mathcal{D}(\gamma,\chi,M)} \mathbb{E}_f\left\{\sup_{\|v\|_2=1}\left|\int_{\mathcal{T}}(v^\top\phi(t))^2dt\right|\sup_t|\hat{f}(t)-f(t)|\right\}^\ell \qquad \text{(S25)}\\
&= \sup_{f\in\mathcal{D}(\gamma,\chi,M)} \mathbb{E}_f\left\{\sup_t|\hat{f}(t)-f(t)|\right\}^\ell\\
&\leq c(r_n+\kappa_{\psi,\infty}(p))^\ell,
\end{aligned}
$$

where the last inequality follows from Proposition 1. Note that

$$
\begin{aligned}
\|(\hat{H}_q+\rho W)^{-1}-(H_q+\rho W)^{-1}\| &\leq \|(I_q+U^{-1}\Delta)^{-1}\|\cdot\|U^{-1}\|^2\cdot\|\Delta\|\\
&\leq c\|(I_q+U^{-1}\Delta)^{-1}\|\cdot\|\Delta\|,
\end{aligned}
$$

where the last inequality is obtained by using Lemma 1. With the assumption $r_n+\kappa_{\psi,\infty}(p)\ll 1$, (S24) then follows from the observation that the probability of the event $\|U^{-1}\Delta\|\leq 1/2$ decays to zero uniformly over the class $\mathcal{F}$ since $r_n+\kappa_{\psi,\infty}(p)\ll 1$. □

# S5 Implementation Details

We collect the procedures outlined in Sections 2.2 and 2.3 into Algorithm 1 with the semi data-driven method for tuning the parameters $q$ and $\rho$. The algorithm is also graphically illustrated in Figure S1. Note that in the algorithm, $G$, $N$, $\hat{\theta}$ and $\hat{a}$ are vectors of length $L$ that grows with $n$, and $G_k$, $N_k$, $\hat{\theta}_k$ and $\hat{a}_k$ represent their elements in the $k$th coordinate. Also note that $q<L$ in general, as $L$ represents the total number of coefficients currently being estimated (including the pre-estimated ones), while $q$ is the number of coefficients currently activated to estimate $\hat{m}$.

# S6 Alternative Tuning Parameter Selection Method

To determine the value of $h$ and choose the tuning parameter $\rho$ in (6), in addition to the semi data-driven strategy described in Section 2.4, another option is to first select $h$ via cross-validation method based on the first $n_0$ observations by minimizing

$$
\mathrm{CV}(h)=\sum_{j=1}^{J}\sum_{i\in\mathscr{P}_j}\{Y_i-\hat{m}^h_{-j}(T_i)\}^2,
$$

**Algorithm 1** Space-saving One-pass Nonparametric Regression

**Inputs:**

Parameters: $C_q$ (default: 1/2), $c_\circ$ (default: 1/2), $q_0$ (default: 5)

Parameters: $h$ and $C_\rho$ set by the semi data-driven method in Section 2.4

Data: A stream of data pairs in batches: $(T_{ij}, Y_{ij})$, $j = 1, \ldots, B$ and $i = 1, 2, \ldots$

**Initialize:**

Predetermine $\{\phi_k\}_{k=1}^\infty$ for estimating the regression function $m$

Predetermine $\{\psi_k\}_{k=1}^\infty$ for estimating the density function $f$

$L \leftarrow q_0$

Set $G$, $N$ and $\hat{\theta}$ to zero vectors of length $L$

Subroutine to maintain the summary statistics:

**for** each $i = 1, 2, \ldots$ **do**

  $n \leftarrow Bi$ ▷ current sample size

  **while** $n \geq \lfloor c_\circ (C_q L)^{1/h} \rfloor$ and there are still available memory units **do**

    $L \leftarrow L + 1$

    Start to pre-estimate $a_L$ by appending a zero entry to each of $G, N, \hat{\theta}$

  **end while**

  **for** $k = 1, 2, \ldots, L$ **do** ▷ update summary statistics

    $G_k \leftarrow G_k + \sum_{j=1}^B \phi_k(T_{ij}) Y_{ij}$

    $\hat{\theta}_k \leftarrow \{N_k \hat{\theta}_k + \sum_{j=1}^B \psi_k(T_{ij})\} / \{N_k + B)\}$

    $N_k \leftarrow N_k + B$

  **end for**

**end for**

Subroutine to answer a query:

**if** a query of estimating $m(t)$ is received for some $t \in \mathcal{T}$ **then**

  $q \leftarrow p \leftarrow \min\{L, \max\{q_0, \lfloor n^h / C_q \rfloor\}\}$

  $\rho \leftarrow C_\rho / n^{(7h+1)/2}$

  $\hat{a} \leftarrow (\hat{H}_q + \rho W)^{-1} N_{1:q}^{-1} G_{1:q}$ ▷ $\hat{H}_q$ is computed in Section 2.2 based on $\hat{\theta}$

  $\hat{m}(t) \leftarrow \sum_{k=1}^q \hat{a}_k \phi_k(t)$

**end if**

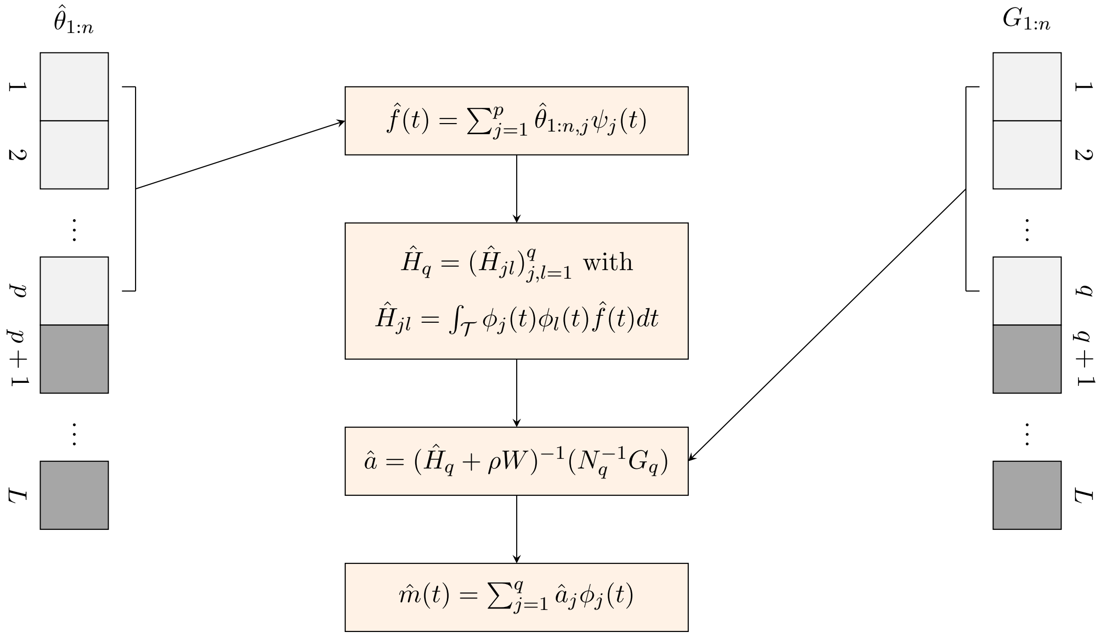


Figure S1: Illustration of the space-saving one-pass estimation procedure (with $p = q$) proposed in Section 2. Here, the dark gray cells represent quantities for pre-estimating $\theta_{p+1}, \ldots$ and $a_{q+1}, \ldots$, while the light gray cells represents summary statistics that are currently used for constructing $\hat{m}$. Note that the quantities in the light orange boxes are not maintained in the memory; instead, they are derived from the summary statistics $\hat{\theta}_{1:n}$ and $G_{1:n}$ in response to a query.

where $\mathscr{P}_1, \ldots, \mathscr{P}_J$ for a positive integer $J$ form a partition of the first $n_0$ observations, and $\hat{m}_{-j}^{h}$ is the estimated regression function without roughness penalty by using the first $q = \lfloor n_0^h / C_q \rfloor$ basis functions and the first $n_0$ observations except those in $\mathscr{P}_j$. The parameter $\rho$ then may be selected in the following fully data-driven and dynamic fashion. When the $n$th batch $\mathscr{D}_n$ of data arrives, for a set of candidate values of $\rho$, we select $\rho$ that minimizes the validation error

$$\mathrm{VE}(\rho) = \sum_{i \in \mathscr{D}_n} \{Y_i - \hat{m}_\rho(T_i)\}^2,$$

where $\hat{m}_\rho$ is the estimated regression function with the value $\rho$ by using the summary statistics derived from the first $n-1$ batches of data. To obtain a stable validation error, a relatively large batch size is required.

We compare the above method with the semi data-driven approach described in Section

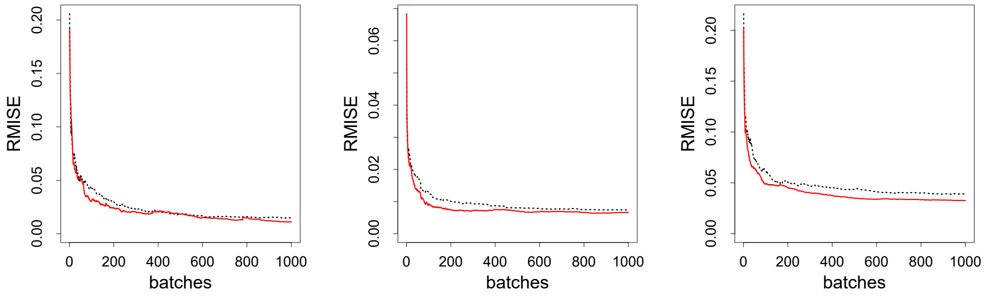


(a) $m_1$ (b) $m_2$ (c) $m_3$

Figure S2: Comparison of the semi data-driven (red solid) and full data-driven (black dotted) methods.

2.4 by using the settings in Section 5.1, and the results displayed in Figure S2 show that they have similar performances. Since the semi data-driven approach is simpler and more robust for data streams of small batch size, it is thus recommended in practice and also adopted in the simulation studies in Section 5.1.

## S7 Numeric Experiments for the Semi Data-driven Strategy

We investigate the impact of the parameters $q_0$ and $C_q$ via additional simulation studies with the settings in Section 5.1 and the following cases:

- $q_0 = 2, 5, 8$ when $C_q = 1/2$;
- $C_q = 2/5, 1/2, 3/5$ when $q_0 = 5$.

The tuning parameters $h$ and $\rho$ are selected by the proposed semi data-driven strategy. The results, displayed in Figures S3 and S4, show that the performance is quite robust to the choice of the parameters $q_0$ and $C_q$ around the recommended values $q_0 = 5$ and $C_q = 1/2$.

## S8 Numeric Experiments on Convergence Rates and Phase Transitions

To numerically validate the convergence rates and phase transitions implied by the theorems and their corollaries in Section 3.3, we reuse the simulation setting for the function

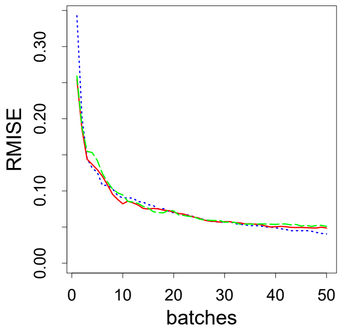


(a) $m_1$ and $n = 1, \ldots, 5000$

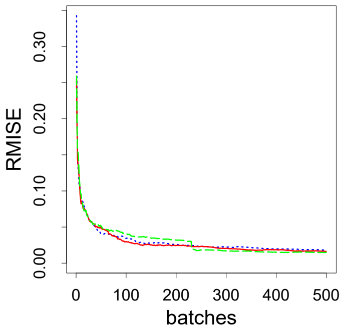


(b) $m_1$ and $n = 1, \ldots, 50000$

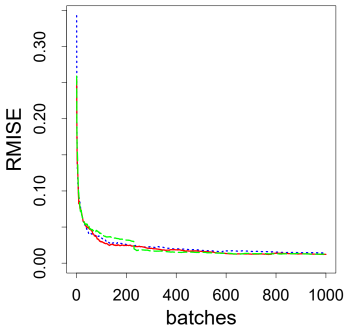


(c) $m_1$ and $n = 1, \ldots, 100000$

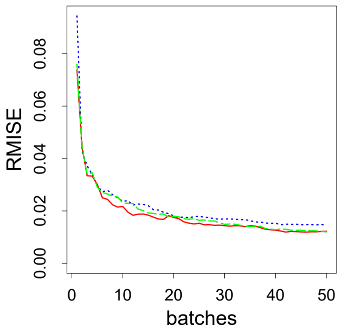


(d) $m_2$ and $n = 1, \ldots, 5000$

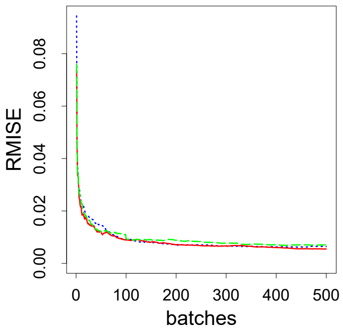


(e) $m_2$ and $n = 1, \ldots, 50000$

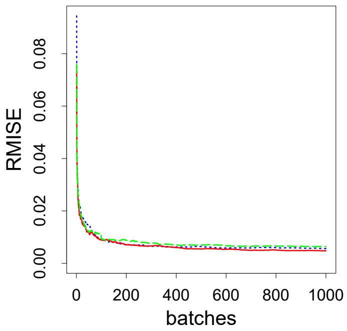


(f) $m_2$ and $n = 1, \ldots, 100000$

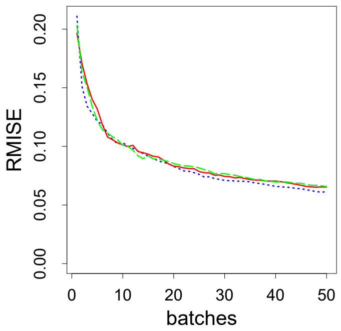


(g) $m_3$ and $n = 1, \ldots, 5000$

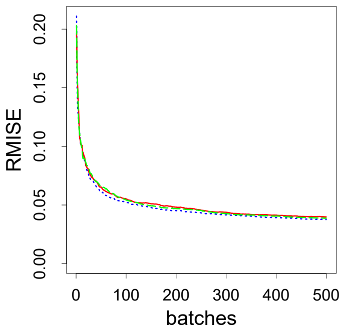


(h) $m_3$ and $n = 1, \ldots, 50000$

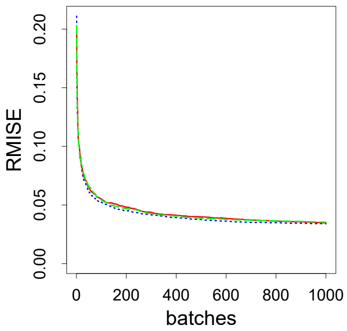


(i) $m_3$ $n = 1, \ldots, 100000$

Figure S3: RMISE based on the first 5000 (left), 50000 (middle) and 100000 (right) observations, for $C_q = 2/5$ (blue dotted), $C_q = 1/2$ (red solid), and $C_q = 3/5$ (green dashed), when $q_0 = 5$ and $h$ is determined by the semi data-driven method.

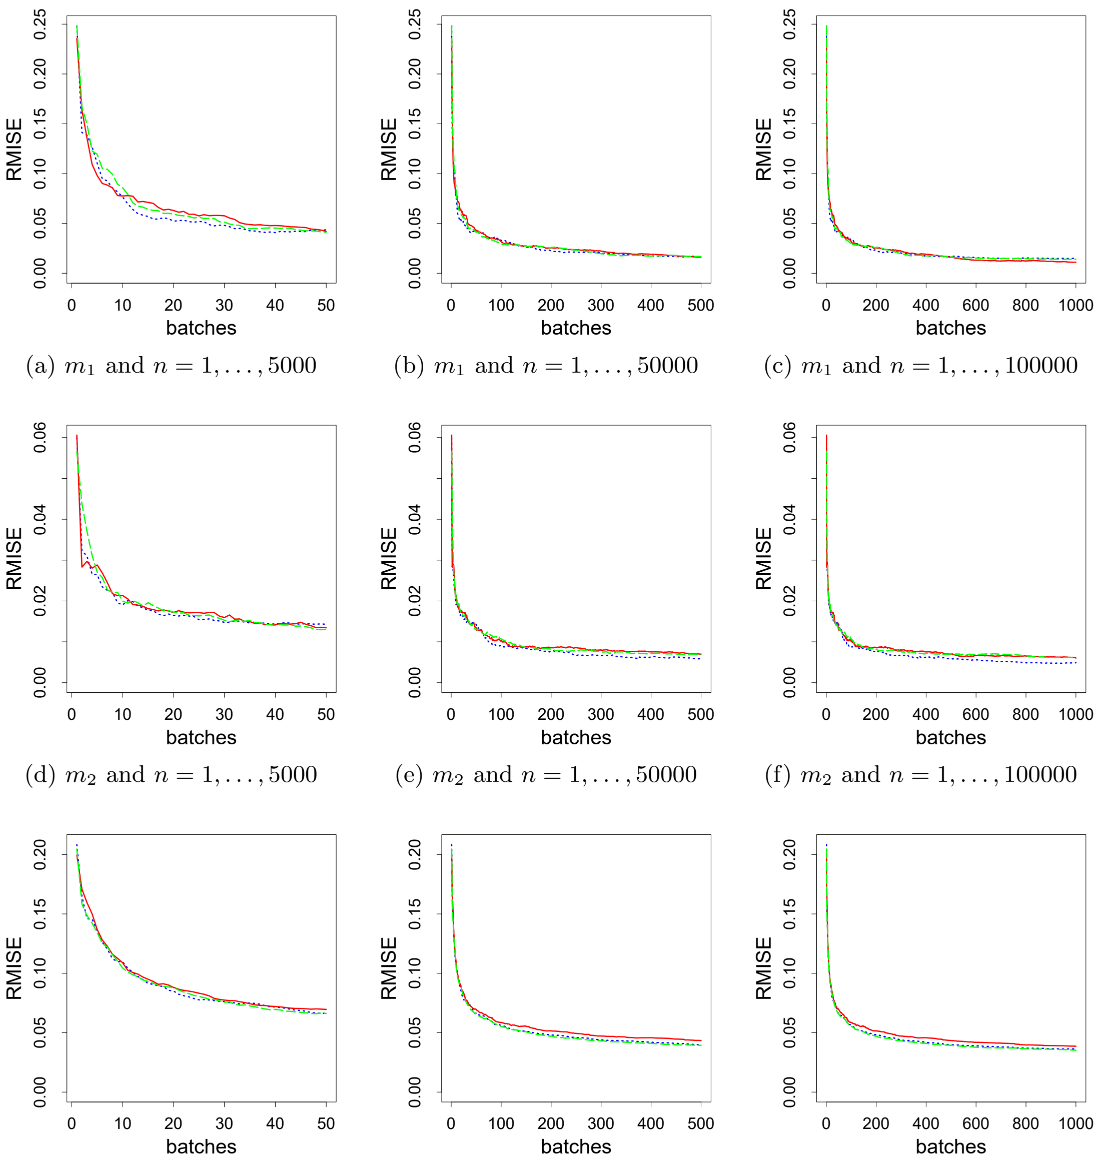


(a) $m_1$ and $n = 1, \ldots, 5000$ (b) $m_1$ and $n = 1, \ldots, 50000$ (c) $m_1$ and $n = 1, \ldots, 100000$

(d) $m_2$ and $n = 1, \ldots, 5000$ (e) $m_2$ and $n = 1, \ldots, 50000$ (f) $m_2$ and $n = 1, \ldots, 100000$

(g) $m_3, n = 1, \ldots, 5000$ (h) $m_3$ and $n = 1, \ldots, 50000$ (i) $m_3$ and $n = 1, \ldots, 100000$

Figure S4: RMISE based on the first 5000 (left), 50000 (middle) and 100000 (right) observations, for $q_0 = 2$ (blue dotted), $q_0 = 5$ (red solid), and $q_0 = 8$ (green dashed), when $C_q = 1/2$ and $h$ is determined by data-driven method.

$m_3(t) = \sum_{k=1}^{\infty} k^{-1.5}\phi_k(t)$ in Section 5.1, where we recall that $\phi_1, \phi_2, \ldots$ are Fourier basis functions. The function $m_3$ is designed in the way that the approximation error by using the first $q$ Fourier basis functions is $\kappa^*_{\phi,2}(m_3, q) \asymp q^{-\beta}$ with $\beta = 1$, where $\kappa^*_{\phi,2}(\cdot,\cdot)$ is defined in Section 3.1. Consequently, a phase transition occurs at $q \asymp n^{1/(2\beta+1)} \asymp n^{1/3}$ for the $L^2$ convergence rate.

In the numeric experiment, we consider $h = 1/5, 1/3, 2/5$ (note that $q := q_n \asymp n^h$) and other parameter settings are the same as the simulation studies in Section 5.1. In addition to RMISE, we also calculate the estimation error $\|\hat{m}_3 - \sum_{k=1}^{q_n} k^{-1.5}\phi_k\|_{L^2}$ and the approximation error $\kappa^*_{\phi,2}(m_3, q_n) = \|\sum_{k=q_n+1}^{\infty} k^{-1.5}\phi_k\|_{L^2}$ for the $L^2$ loss function. The corresponding results based on 100 independent Monte Carlo replicates are presented in Figures S5 and S6, as well as Table S1 for $h = 1/3$. As expected, Figure S5 shows that, for all sufficiently large $n$, the approximation error is much larger than the estimation error when $h = 1/5$, the situation is reversed when $h = 2/5$, and the two errors are roughly of the same magnitude when $h = 1/3$. Similar patterns are observed in Figure S6 for the uniform convergence with the estimation error $\|\hat{m}_3 - \sum_{k=1}^{q_n} k^{-1.5}\phi_k\|_\infty$ and the approximation error $\kappa^*_{\phi,\infty}(m_3, q_n) = \|\sum_{k=q_n+1}^{\infty} k^{-1.5}\phi_k\|_\infty$.

As it is difficult to calculate the precise constants hidden inside $O_P$ of the corollaries in Section 3.3, to validate the convergence rates, for the $L^2$ convergence, we consider the empirical ratio $\|\hat{m}_{3,n_1} - m_3\|_{L^2}/\|\hat{m}_{3,n_2} - m_3\|_{L^2}$ for two different sample sizes $n_1$ and $n_2$ to get rid of the hidden constants, where $\hat{m}_{3,n}$ is the proposed estimator $\hat{m}_3$ for $m_3$ when the sample size is $n$. According to Corollary 4, the theoretically predicted ratio should be close to $n_1^{-\beta/(2\beta+1)}/n_2^{-\beta/(2\beta+1)} = (n_1/n_2)^{-1/3}$ since $\beta = 1$ for $m_3$. For the uniform convergence, we consider the similar ratio $\|\hat{m}_{3,n_1} - m_3\|_\infty/\|\hat{m}_{3,n_2} - m_3\|_\infty$ and the theoretically predicted ratio is $(n_1/n_2)^{-1/3}(\log n_1/\log n_2)^{1/3}$. If the rates in the corollaries of Section 3.3 are correct and tight, then we expect the empirical ratios (with the optimal choice $h = 1/(2\beta+1) = 1/3$ for estimating $m_3$) to be closer to their theoretical counterparts as $n \to \infty$. This is indeed the result observed from Table S1, and thus numerically validates the established asymptotic convergence rates.

## S9 Numeric Impact of Density Function

In Theorems 1 and 2, the assumption $\kappa_{\phi,\infty}(q) \lesssim 1$ and $\kappa_{\psi,\infty}(p) \ll 1$ implicitly requires the density function $f$ to be smoother than the regression function $m$. In addition, the conditions "$\gamma \geq \beta + 1/2$" in Corollary 2 and "$\gamma > \beta > 0$" in Corollary 4 make this

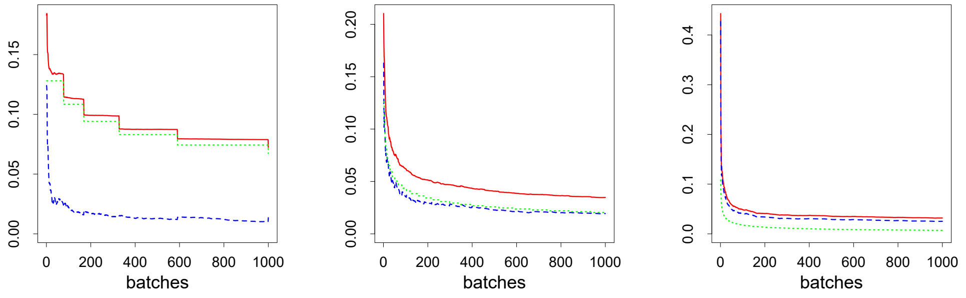


(a) $h = 1/5$ (b) $h = 1/3$ (c) $h = 2/5$

Figure S5: Empirical RMISE (red solid), estimation errors (blue dashed), and approximation errors (green dotted) under different growth rates of $q$.

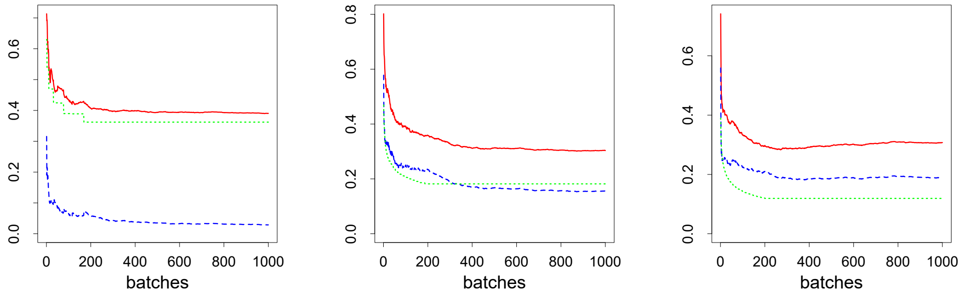


(a) $h = 1/5$ (b) $h = 1/3$ (c) $h = 2/5$

Figure S6: Empirical uniform errors (red solid), estimation errors (blue dashed), and approximation errors (green dotted) under different growth rates of $q$.

| $n_1/n_2$ | $L^2$ Convergence | | Uniform Convergence | |
|---|---|---|---|---|
| | theoretical | empirical | theoretical | empirical |
| 25000/5000 | 0.585 | 0.625 | 0.620 | 0.685 |
| 50000/10000 | | 0.603 | 0.617 | 0.654 |
| 100000/20000 | | 0.589 | 0.615 | 0.624 |

Table S1: Comparison of the theoretical and empirical convergence rates in terms of $\|\hat{m}_{3,n_1} - m_3\|_{L^2}/\|\hat{m}_{3,n_2} - m_3\|_{L^2}$ for the $L^2$ convergence and $\|\hat{m}_{3,n_1} - m_3\|_\infty/\|\hat{m}_{3,n_2} - m_3\|_\infty$ for the uniform convergence. The theoretical ratios for the $L^2$ convergence are constant since $n_1$ and $n_2$ are chosen in the way that $n_1/n_2 = 5$ for all three cases. For the uniform convergence, the theoretical ratios are not constant due to the additional $(\log n_1/\log n_2)^{1/3}$ factor that stems from the $\log n$ factor of the optimal uniform convergence rate in Corollary 2.

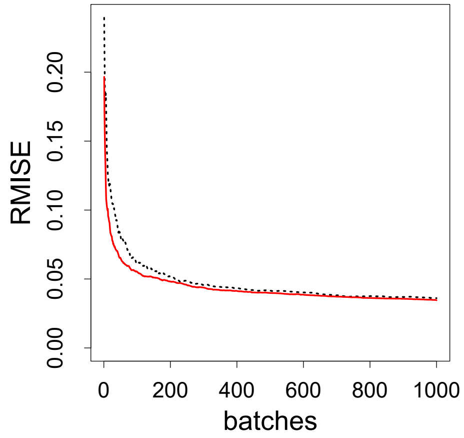


Figure S7: RMISE of the proposed estimator for $m_3$ with the uniform density function (red solid) and the alternative density function (black dotted) defined in Eq (S26) .

requirement explicit.

To investigate the numeric impact of this smoothness assumption on the density function, we conduct an additional numeric experiment by reusing the setting of $m_3$ in Section 5.1 and considering the density

$$f(t) = A_f \sum_{k=1}^{\infty} k^{-0.8} \phi_k(t) \tag{S26}$$

for some constant $A_f$ that makes $f$ into a bona fide density function on $[0, 1]$, where $\phi_1(t) = 1$, $\phi_{2k}(t) = \cos(2k\pi t)$ and $\phi_{2k+1}(t) = \sin(2k\pi t)$ for $k \geq 1$; note that this density function is positive on $[0, 1]$. As $\kappa^*_{\phi,2}(f, q) \asymp q^{-\gamma}$ with $\gamma = 3/10 < \beta$, the function $f$ is less smooth than $m_3$ with $\beta = 1$. In the experiment, the data are generated and the tuning parameters are selected in the same way of the studies in Section 5.1, except that now the predictors are drawn from the distribution induced by the above density function $f$. We then compare the RMISE of the estimated $\hat{m}_3$ in this case with the one with the uniform density function, and find in Figure S7 that both density functions lead to almost identical RMISE in the long run. This suggests, certain violation of the smoothness assumption on the density function has limited impact on the asymptotic numeric performance of the proposed estimator.

## S10 Comparison on Computation Time

In the streaming setting, there are two types of computation time: the maintenance time for processing a batch of data and updating the summary statistics, and the query time for producing an estimate of $m(t)$ for a given $t$ based on the summary statistics. Figure S8 provides a comparison on these two types of computation time required by the proposed method, OPLS and DPSR for the simulation studies in Section 5.1. Note that both OPLS and the proposed method need to compute some quantities by using the first few batches of data, such as the constant $\theta_\mu$ of OPLS (defined in Appendix B, Yang and Yao, 2022) and $h$ of the proposed method, and thus a spike of the maintenance time at the beginning of the stream is observed for each of these two methods in Figure S8.

The comparison shows that, the proposed method is as efficient as DPSR in terms of computation time for updating summary statistics, and much faster than DPSR for answering a query, especially in the long run. More specifically, the query time of both the proposed method and DSPR grows with the sample size $n$, with the proposed method having a substantially slower growth rate and a visibly lower start of the query time, as it uses relatively less basis functions than DSPR.

As per Remark 2, we need to specify a set of fixed points before running the OPLS algorithm, and the maintenance time of OPLS showed in Figure S8 is for updating the local statistics for $\ell = 100$ fixed points. A smaller value of $\ell$ can linearly reduce the maintenance time of OPLS, at the cost of reduced ability to answer queries, since OPLS can only produce estimates at these fixed points and thus less fixed points lead to less queries that OPLS can answer. On the other hand, OPLS is observed to spend nearly constant time on answering a query about an estimate at a predetermined fixed point. This computational feature of OPLS may make it suitable for applications where the volume of queries is much larger than the data volume and all queries are about estimates of $m(t)$ for a predetermined small set of fixed points $t \in \mathcal{T}$. Otherwise, the proposed method may be preferred due to its efficiency in both computation time and memory as well as its ability to produce an estimate of $m(t)$ for an arbitrary $t \in \mathcal{T}$ in any time of the streaming process.

## S11 Fourier Extension

When a non-periodic function $g(t)$, $t \in \mathcal{T}$, is approximated by the first $q$ Fourier basis functions, the estimator $\hat{g}(t)$ often exhibits drastic oscillatory overshoot around the

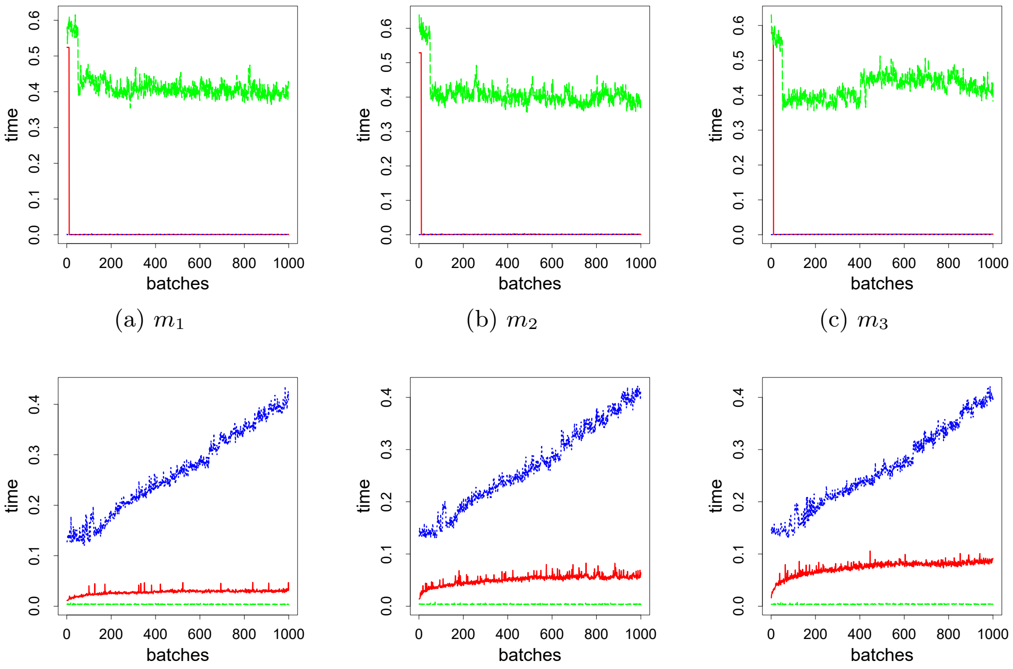


(a) $m_1$ (b) $m_2$ (c) $m_3$

(d) $m_1$ (e) $m_2$ (f) $m_3$

Figure S8: Average maintenance time (top) for processing each data batch and the average query time (bottom) for answering 100 queries, in seconds, for the proposed method (red solid), the OPLS method (green dashed), and the DPSR method (blue dotted) based on 100 independent Monte Carlo replicates.

boundaries of the domain, which is called the Gibbs phenomenon. To achieve a stabler estimator, the recently developed Fourier extension technique (Adcock et al., 2014) may be adopted. The basic idea is to extend the original domain by a margin $\mu > 0$. Take $\mathcal{T} = [0, 1]$ for illustration. The extended domain is $[-\mu, 1 + \mu]$. In the extended domain, a new sequence of extended basis functions $\eta_1(t), \eta_2(t), \dots$ is defined, specifically, by $\eta_1(t) = (1+2\mu)^{-1/2}$, $\eta_{2k}(t) = \cos\{2\pi t/(1+2\mu)\}$ and $\eta_{2k+1}(t) = \sin\{2\pi t/(1+2\mu)\}$ for $k \geq 1$. Let $\mathcal{G}_q(\mu) = \text{span}\{\eta_1, \eta_2, \dots, \eta_q\}$. The best approximate $\tilde{g}$ of the function $g$ within $\mathcal{G}_q(\mu)$ is defined by

$$\tilde{g} = \underset{h \in \mathcal{G}_q(\mu)}{\arg\min} \|g - h\|_{L^2(0,1)}.$$

Note that in the above the $L^2$ norm is calculated only over the original domain. Numerical studies show that, by adopting the Fourier extension with $\mu$ set to 10% of the length of the original domain, the Gibbs phenomenon appears only prominently in the boundary areas $[-\mu, 0]$ and $[1, 1+\mu]$, so that we avoid overshoot within the original domain $[0, 1]$. In addition, this approximate $\tilde{g}$ enjoys the same theoretical convergence rate of the approximate by the non-extended Fourier basis functions. For instance, if the function $g$ is $\beta$ times continuously differentiable, then $\tilde{g}$ converges to $g$ in the $L^2(0, 1)$ norm at the rate $q^{-\beta}$ (Adcock et al., 2014).

# References


Adcock, B., Huybrechs, D., and Martín-Vaquero, J. (2014). On the numerical stability of fourier extensions. *Foundations of Computational Mathematics*, 14(4):635–687.

Chen, X. and Christensen, T. M. (2015). Optimal uniform convergence rates and asymptotic normality for series estimators under weak dependence and weak conditions. *Journal of Econometrics*, 188(2):447–465.

Deadman, E. and Relton, S. D. (2016). Taylor's theorem for matrix functions with applications to condition number estimation. *Linear Algebra and its Applications*, 504:354–371.

Ding, X. and Zhou, Z. (2020). Estimation and inference for precision matrices of nonstationary time series. *The Annals of Statistics*, 48(4):2455–2477.

Minsker, S. (2017). On some extensions of Bernstein's inequality for self-adjoint operators. *Statistics & Probability Letters*, 127:111–119.

Yang, Y. and Yao, F. (2022). Online estimation for functional data. *Journal of the American Statistical Association*, page to appear.
